# Supplementary material for: Physics-Free Spectrally Multiplexed Photometric Stereo under Unknown Spectral Composition
Source: arXiv:2410.20716 source file (2024-10-28)
Supplement: Supplementary file 1 [file ablation.tex]

\section{Ablation Study using Synthetic Dataset}
\label{sec:supp_ablation}
In this section, we validate the individual technical contributions of our training dataset (\ie, PS-Multiplex) and the physics-free architecture (\ie, SpectraM-PS) using a synthetic evaluation dataset. 
Firstly, we validate the efficacy of our training dataset, PS-Multiplex, by adapting an existing universal photometric stereo architecture designed for the conventional task (\ie, SDM-UniPS~\cite{Ikehata2023}) to the spectrally multiplexed photometric stereo task. Since both ours and SDM-UniPS take multiple observations and an object mask as input, this adaptation straightforwardly involves training the model on PS-Multiplex by treating each channel of an image as an individual image. Subsequently, we compare this model against our proposed SpectraM-PS to demonstrate the efficacy of our dual-scale design with local patch embedding.

For a more analytical discussion, instead of using SMuP for this study, we additionally rendered three-channel spectrally multiplexed images representing six distinct surface material categories: (a) uniform, Lambertian; (b) piece-wise uniform, Lambertian; (c) non-uniform, Lambertian; (d) uniform, non-Lambertian; (e) piece-wise uniform, non-Lambertian; and (f) non-uniform, non-Lambertian. In uniform materials, every point on the surface within a scene exhibits the same material properties. For piece-wise uniform materials, each object in a scene is composed of the same material, yet different objects possess distinct materials. Non-uniform materials feature unique PBR textures assigned to each object. Regarding Lambertian scenes, the roughness parameter is set to one in the Principled BSDF~\cite{DisneyPrincipledBSDF}. Conversely, in non-Lambertian scenes, roughness maps derived from PBR textures are utilized for the Principled BSDF.~\cref{fig:synthetic} displays examples of these materials and their corresponding rendered images. The rendering process for these images was identical to that used for the PS-Multiplex datasets in each category. We generated 100 scenes for each surface material category, and results (\ie, MAE) are averaged over them, with each featuring three overlapping objects. The objects and materials were randomly chosen from AdobeStock~\cite{AdobeStock}, and the illumination conditions were randomly selected from four different setups (\ie, point, point+directional, point+environment, environment). Each scene was rendered as a $512\times512$ 16-bit image, along with a ground truth surface normal map. It is crucial to note that the data creation process was entirely independent for each material category, rendering it inappropriate to compare average angular errors across different material categories for meaningful insights.

The results are presented in~\cref{table:uniform}, \cref{table:piecewise}, and\cref{table:nonuniform}. Consistent results were observed across different surface conditions. In summary, the universal photometric stereo method~\cite{Ikehata2023} trained on our PS-Multiplex dataset demonstrates proper adaptation to the spectrally multiplexed photometric stereo task. Nonetheless, our SpectraM-PS method significantly enhanced reconstruction accuracy, showcasing an architecture-level improvement over SDM-UniPS for the spectrally multiplexed photometric stereo task, where the number of input channels is typically much fewer than that of input images for temporally-multiplexed photometric stereo.

To qualitatively demonstrate the advantage of our SpectraM-PS with fewer input channels over SDM-UniPS~\cite{Ikehata2023}, we extended its application to the conventional photometric stereo task. This task featured six images captured under a single white area LED light source, illustrating that our method can also be applied to the temporally multiplexed photometric stereo task by treating images (averaged to a grayscale image) as independent channels even though the model is entirely trained on PS-Multiplex. As depicted in~\cref{fig:alligator}, our surface normal decoder, adept at leveraging local patch statistics, exhibited superior performance in recovering fine surface details.

\begin{figure}[t]
	\begin{center}
		\includegraphics[width=120mm]{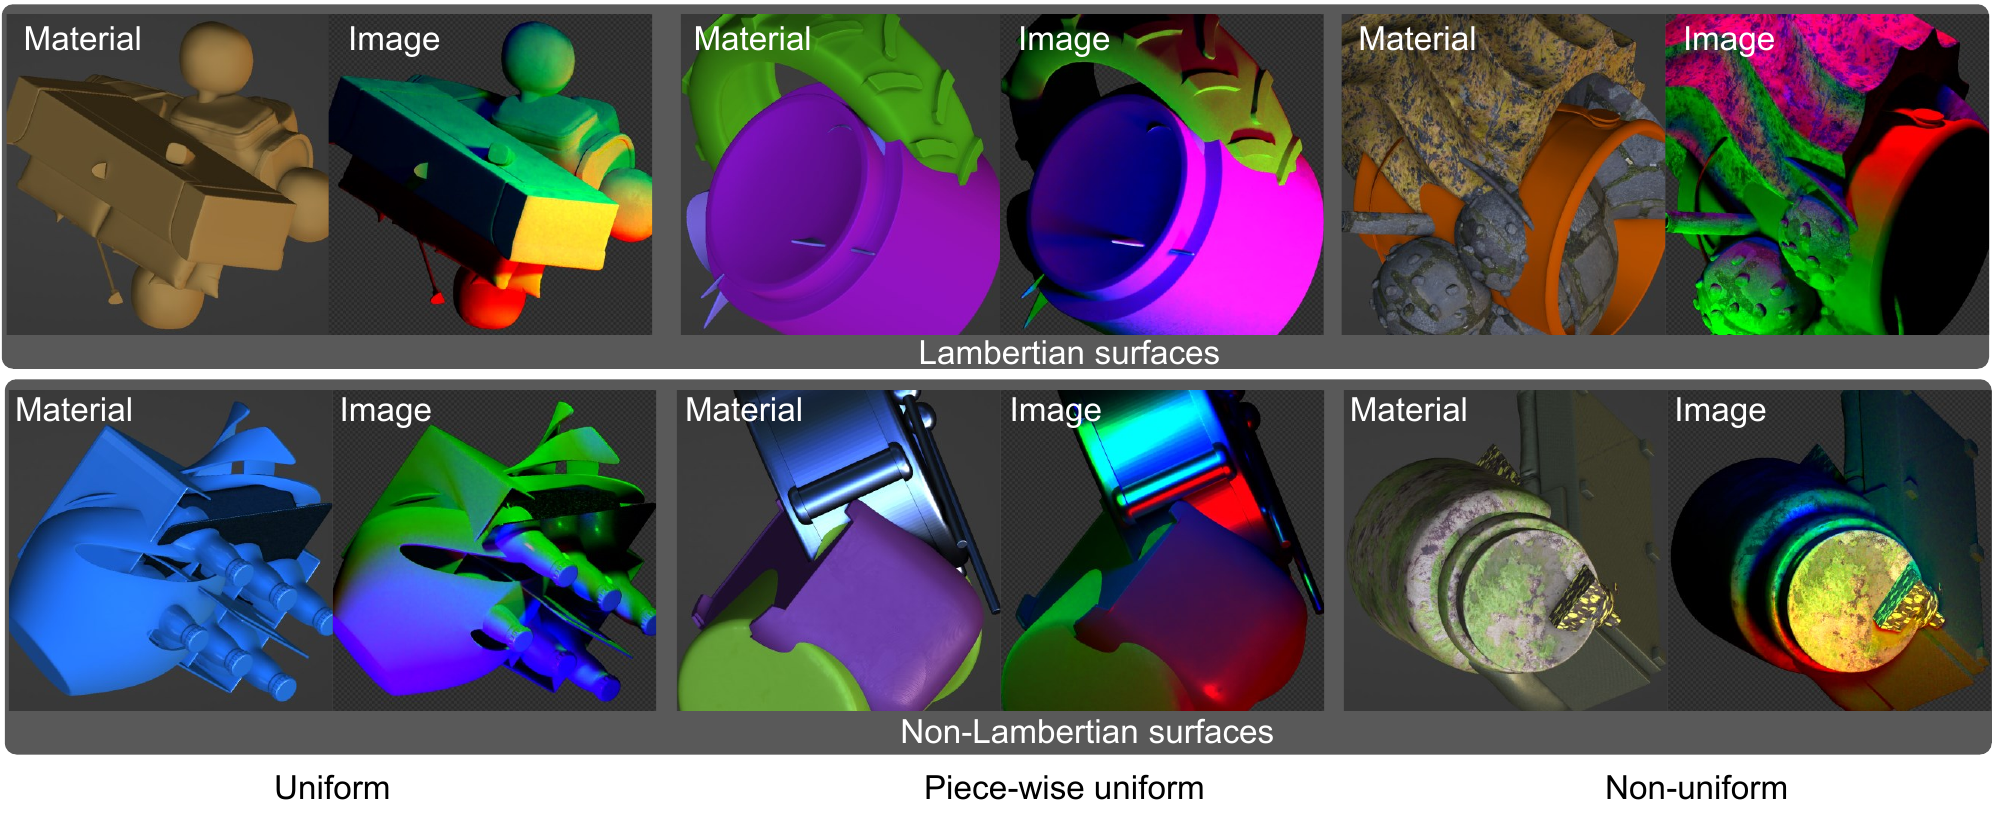}
	\end{center}
	\vspace{-5pt}
	\caption{Examples in synthetic evaluation datasets.}
	\vspace{-10pt}
	\label{fig:synthetic}
\end{figure}

\begin{table}[!t]
\setlength{\tabcolsep}{2.5mm} 
    \centering
    \caption{Ave.(Std.) of MAE (Uniform) over 100 scenes.}
    \small
    \begin{tabularx}{100mm}{cXX}
    \toprule
    Method & Non-Lambertian & Lambertian\\
    \midrule
    SDM-UniPS~\cite{Ikehata2023} & 12.9 (4.5) & 12.4 (4.7) \\
    \cite{Ikehata2023} trained on PS-Multiplex & 11.1 (3.6) & 11.0 (3.9)\\
    SpectraM-PS (Ours) & \textbf{8.0} (2.7) &  \textbf{8.4} (2.7)\\
    \bottomrule
    \end{tabularx}
    \label{table:uniform}
\end{table}
\begin{table}[!t]
\setlength{\tabcolsep}{2.5mm} 
    
    \centering
    \caption{Ave.(Std.) of MAE (Piece-wise uniform) over 100 scenes.}
    \small
    \begin{tabularx}{100mm}{cXX}
    \toprule
    Method & Non-Lambertian & Lambertian\\
    \midrule
    SDM-UniPS~\cite{Ikehata2023} & 15.0 (5.0) & 21.7 (7.0) \\
    \cite{Ikehata2023} trained on PS-Multiplex & 10.5 (2.9) & 12.3 (3.9)\\
    SpectraM-PS (Ours) & \textbf{7.9} (2.4) &  \textbf{8.9} (2.9)\\
    \bottomrule
    \end{tabularx}
    \label{table:piecewise}
\end{table}
\begin{table}[!t]
\setlength{\tabcolsep}{2.5mm}     
    \centering
    \caption{Ave.(Std.) of MAE (Non-uniform) over 100 scenes.}
    \small
    \begin{tabularx}{100mm}{cXX}
    \toprule
    Method & Non-Lambertian & Lambertian\\
    \midrule
    SDM-UniPS~\cite{Ikehata2023} & 14.4 (5.1) & 15.2 (5.9) \\
    \cite{Ikehata2023} trained on PS-Multiplex & 10.6 (3.9) & 11.2 (3.7)\\
    SpectraM-PS (Ours) & \textbf{8.2} (3.2) &  \textbf{8.0} (2.5)\\
    \bottomrule
    \end{tabularx}
    \label{table:nonuniform}
\end{table}
\begin{figure}[!t]
	\begin{center}
		\includegraphics[width=120mm]{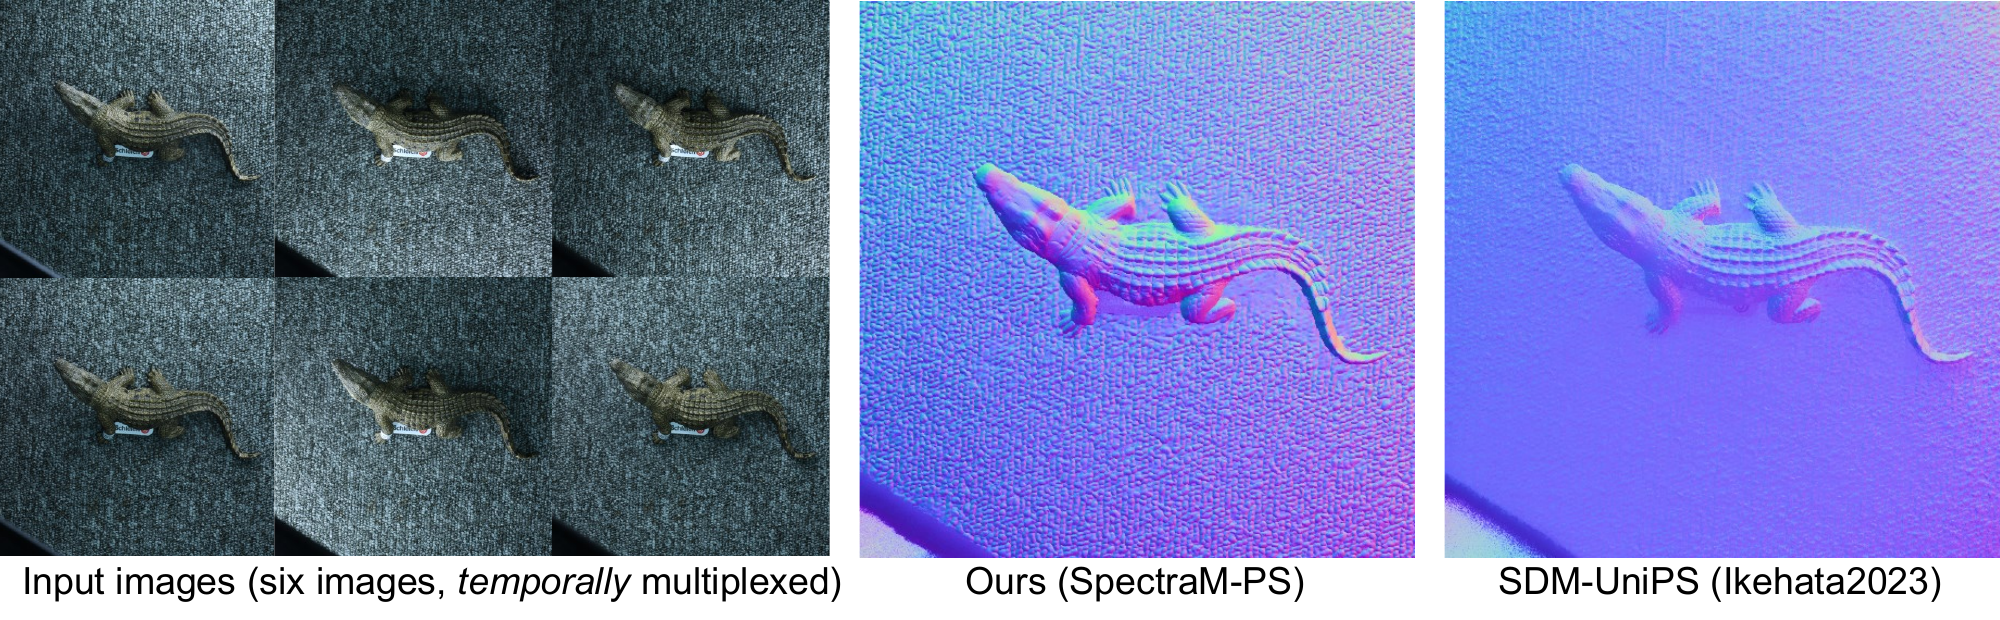}
	\end{center}
	\vspace{-10pt}
	\caption{We applied both SpectraM-PS, trained on PS-Multiplex (our method), and SDM-UniPS, trained on PS-Mix~\cite{Ikehata2023}, to images captured under six white LEDs (\ie, temporally multiplexed). We observed that the surface normal map recovered by our method significantly retained fine details on both the carpet and the alligator's surface, whereas SDM-UniPS failed to produce satisfactory detail.}
	\label{fig:alligator}
	\vspace{-5pt}
\end{figure}
