# Supplementary material for: Physics-Free Spectrally Multiplexed Photometric Stereo under Unknown Spectral Composition
Source: arXiv:2410.20716 source file (2024-10-28)
Supplement: Supplementary file 2 [file object.tex]

\section{Details of SMuP Objects}\label{sec:supp_object}
Here, we provide more information about the objects in our dataset. The appearance of each object under a white light source and the intensity distribution information of the image data in the dataset are shown in~\cref{fig:objects_histogram_astranout} $\sim$~\cref{fig:objects_histogram_tree}. A variety of objects are included in our dataset, ranging from those with monochrome colors to multicolored ones, and from those with Lambertian reflective properties to those with strong specular reflective properties. Please refer to the figure captions for details on reflective properties.

\begin{figure}[h]
	\begin{center}
		\includegraphics[width=120mm]{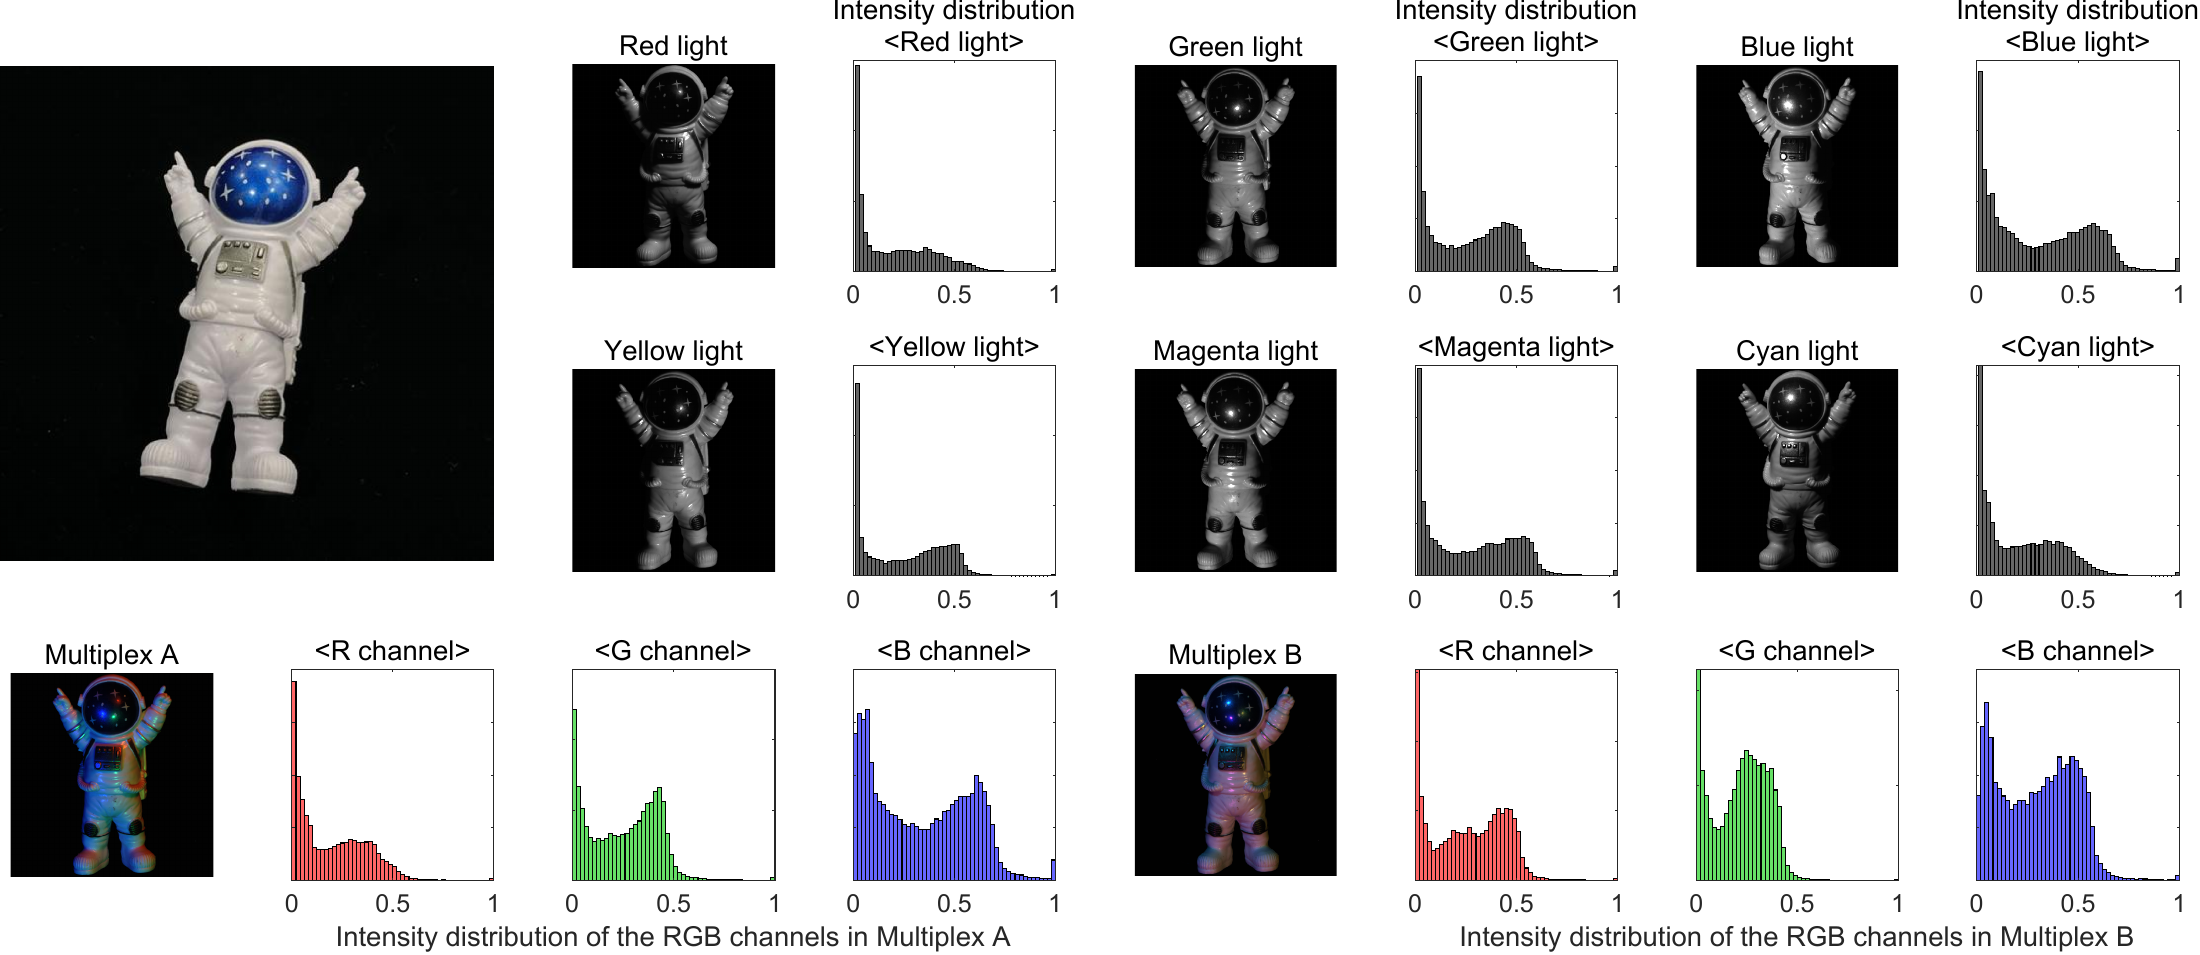}
	\end{center}
	\vspace{-15pt}
	\caption{Astronaut.
 \protect\linebreak Reflective properties : broad and soft specular lobes.}
	\label{fig:objects_histogram_astranout}
	\vspace{-5pt}
\end{figure}

\begin{figure}[h]
	\begin{center}
		\includegraphics[width=120mm]{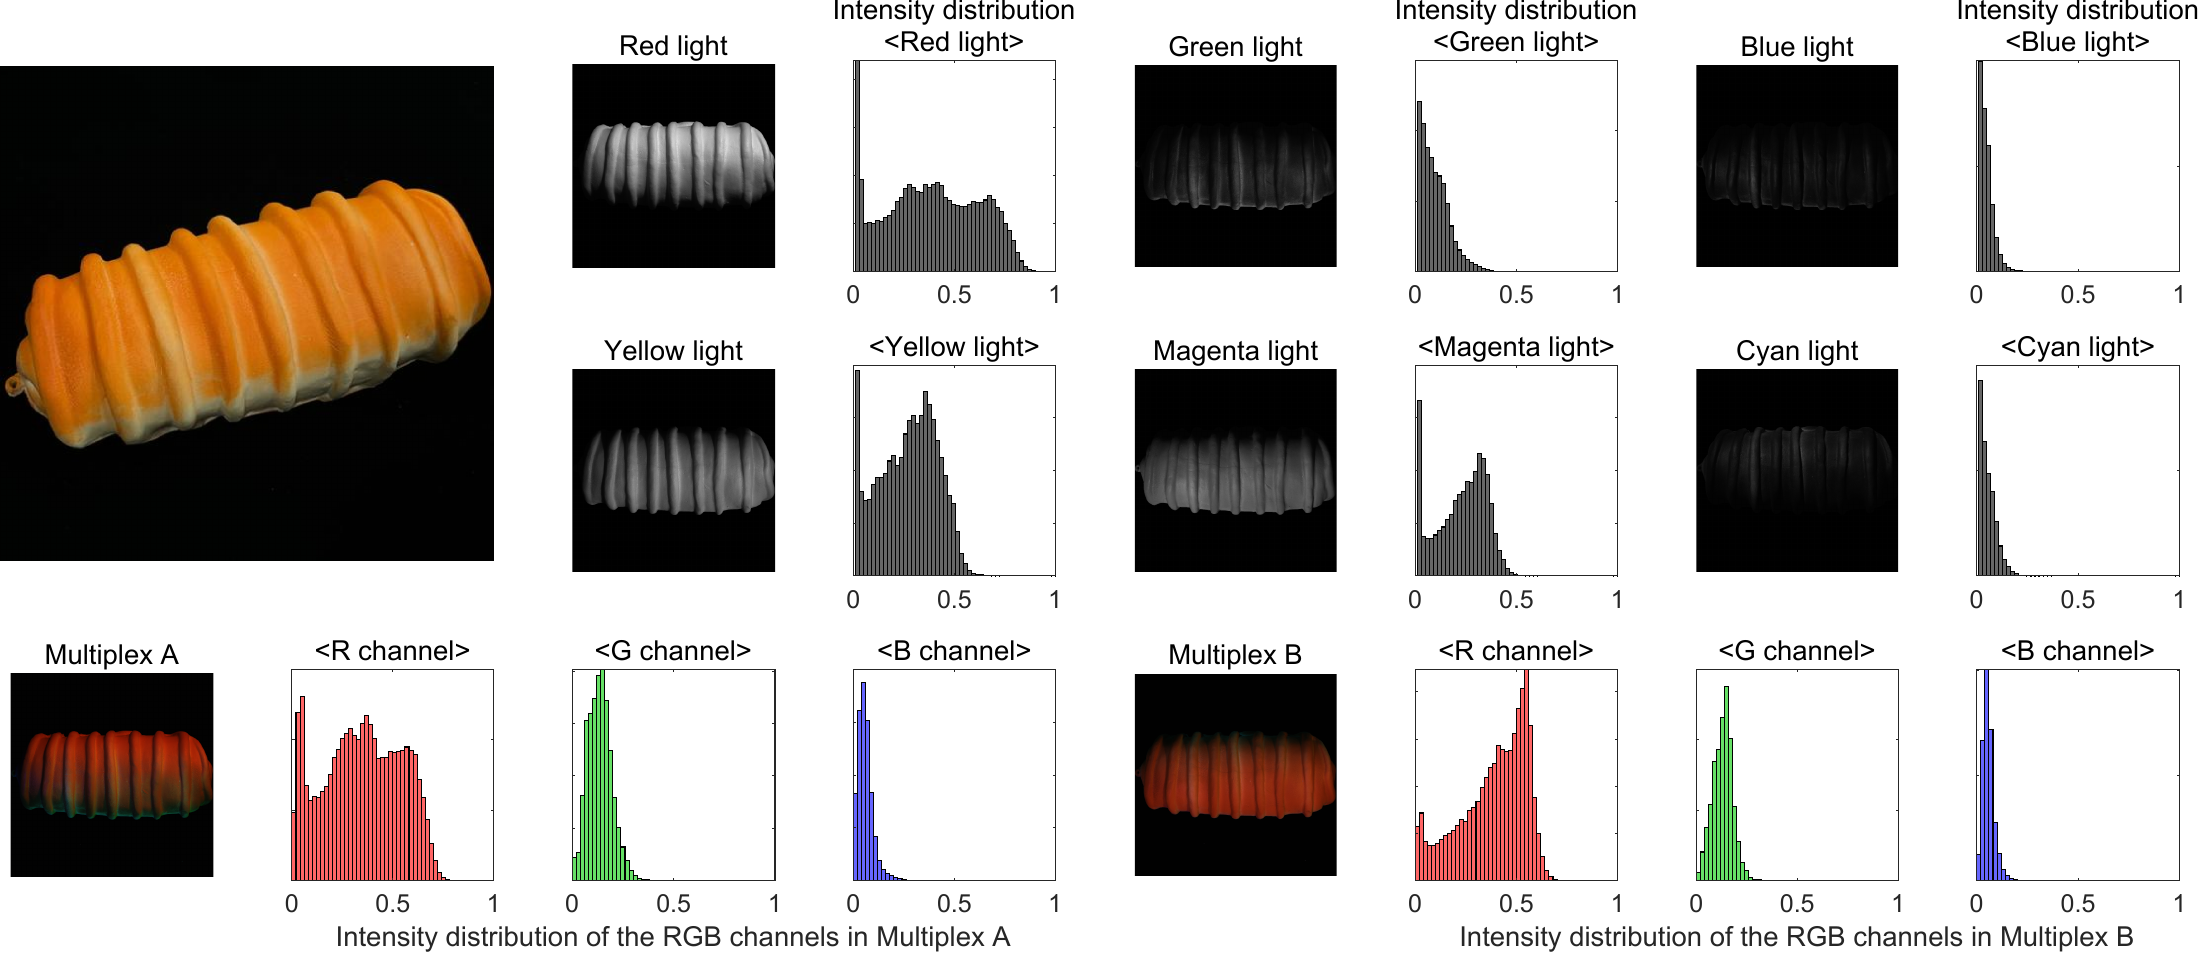}
	\end{center}
	\vspace{-15pt}
	\caption{Bread.
 \protect\linebreak Reflective properties : mostly diffuse.}
	\label{fig:objects_histogram_bread}
	\vspace{-5pt}
\end{figure}

\begin{figure}[h]
	\begin{center}
		\includegraphics[width=120mm]{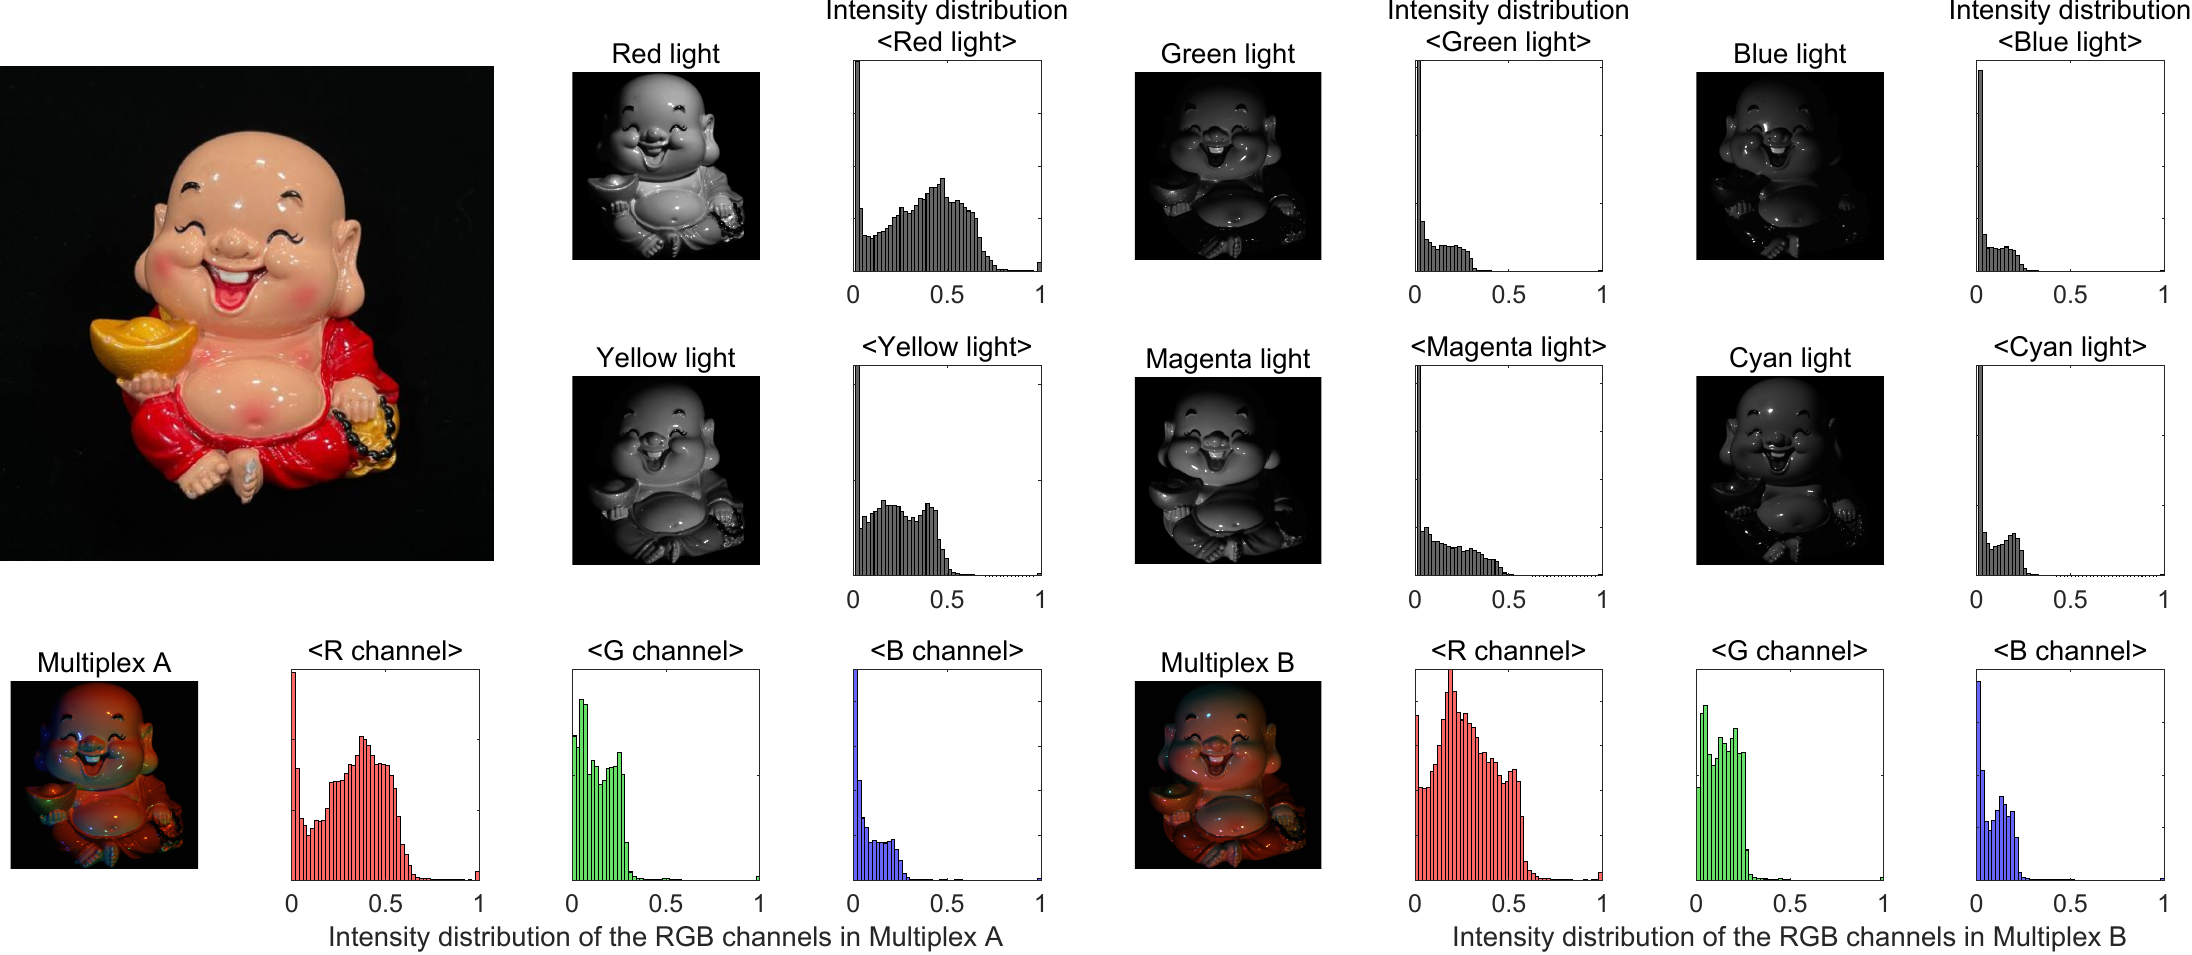}
	\end{center}
	\vspace{-15pt}
	\caption{Buddha.
 \protect\linebreak Reflective properties : strong and sparse specular spikes.}
	\label{fig:objects_histogram_buddha}
	\vspace{-5pt}
\end{figure}

\begin{figure}[h]
	\begin{center}
		\includegraphics[width=120mm]{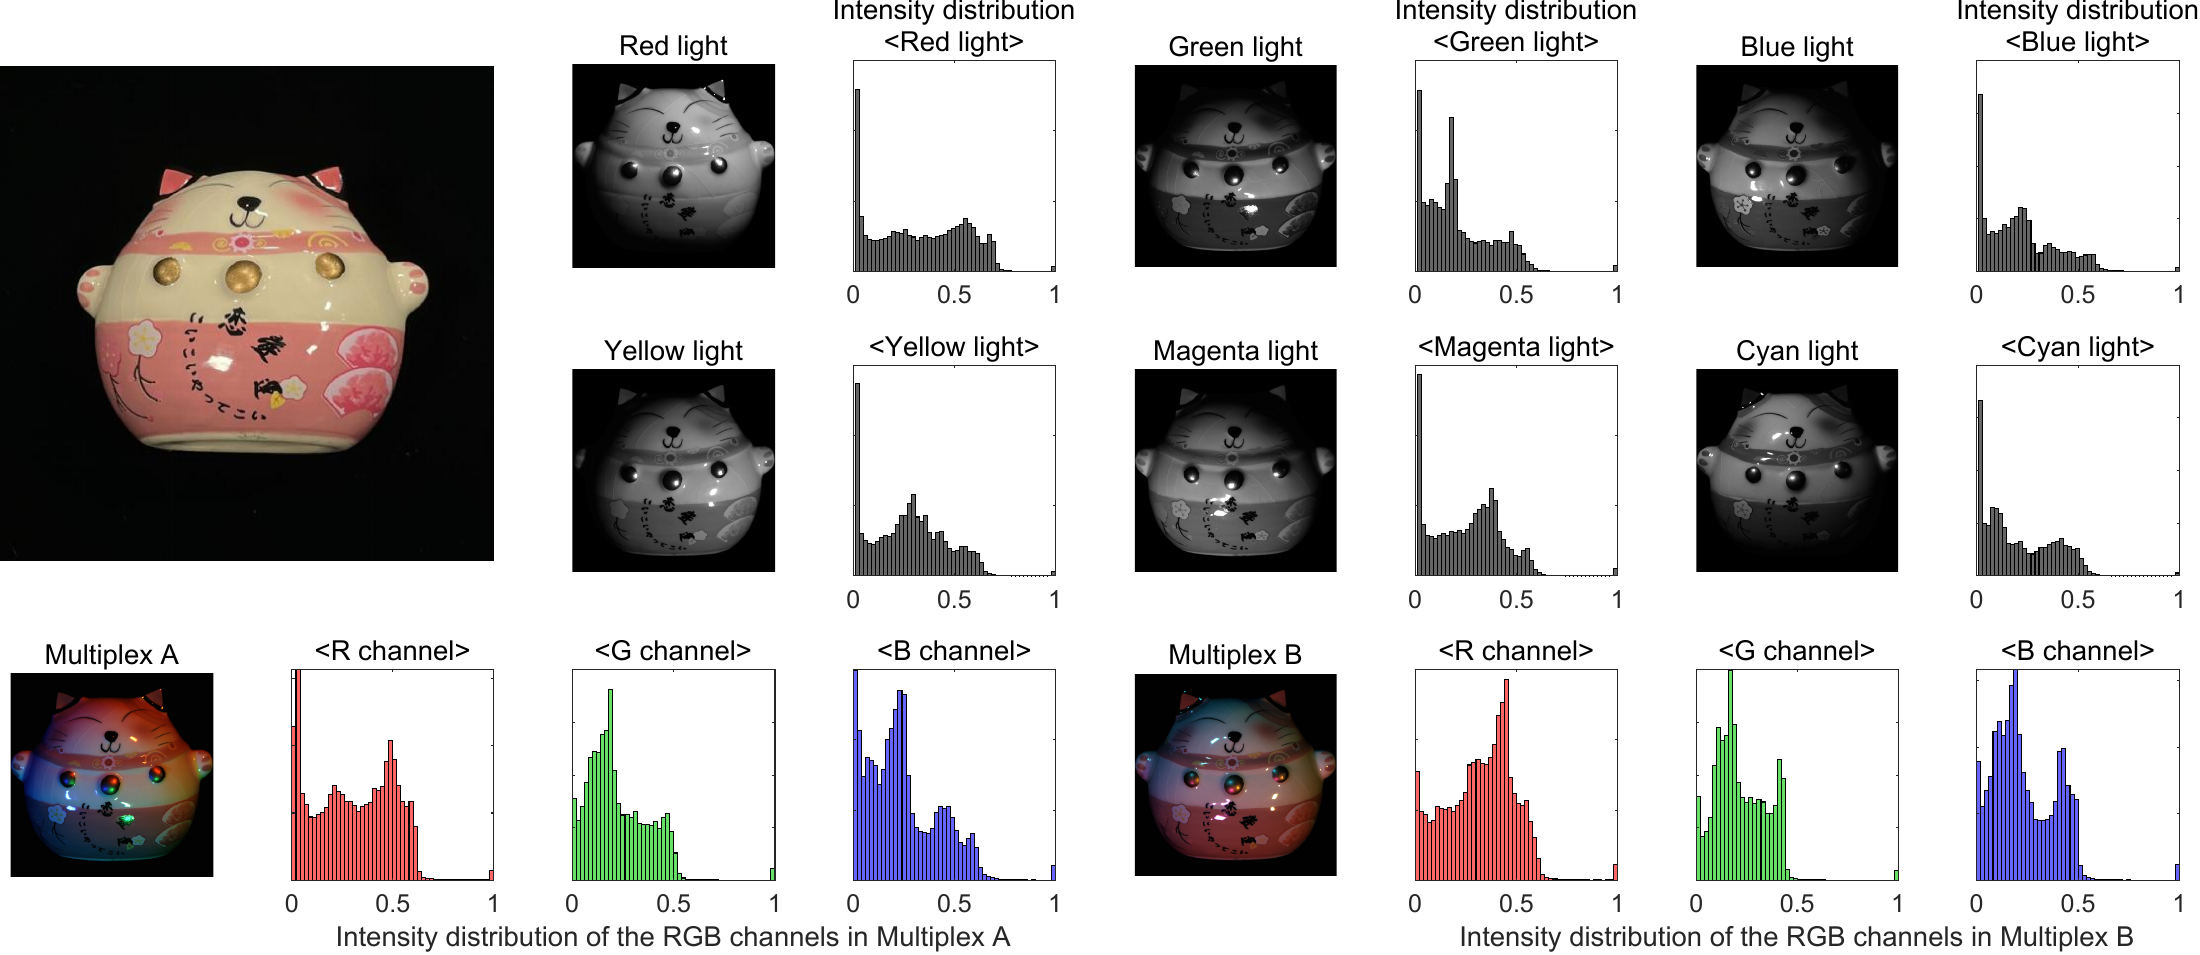}
	\end{center}
	\vspace{-15pt}
	\caption{Cat.
 \protect\linebreak Reflective properties : strong and sparse specular spikes.}
	\label{fig:objects_histogram_cat}
	\vspace{-5pt}
\end{figure}

\begin{figure}[h]
	\begin{center}
		\includegraphics[width=120mm]{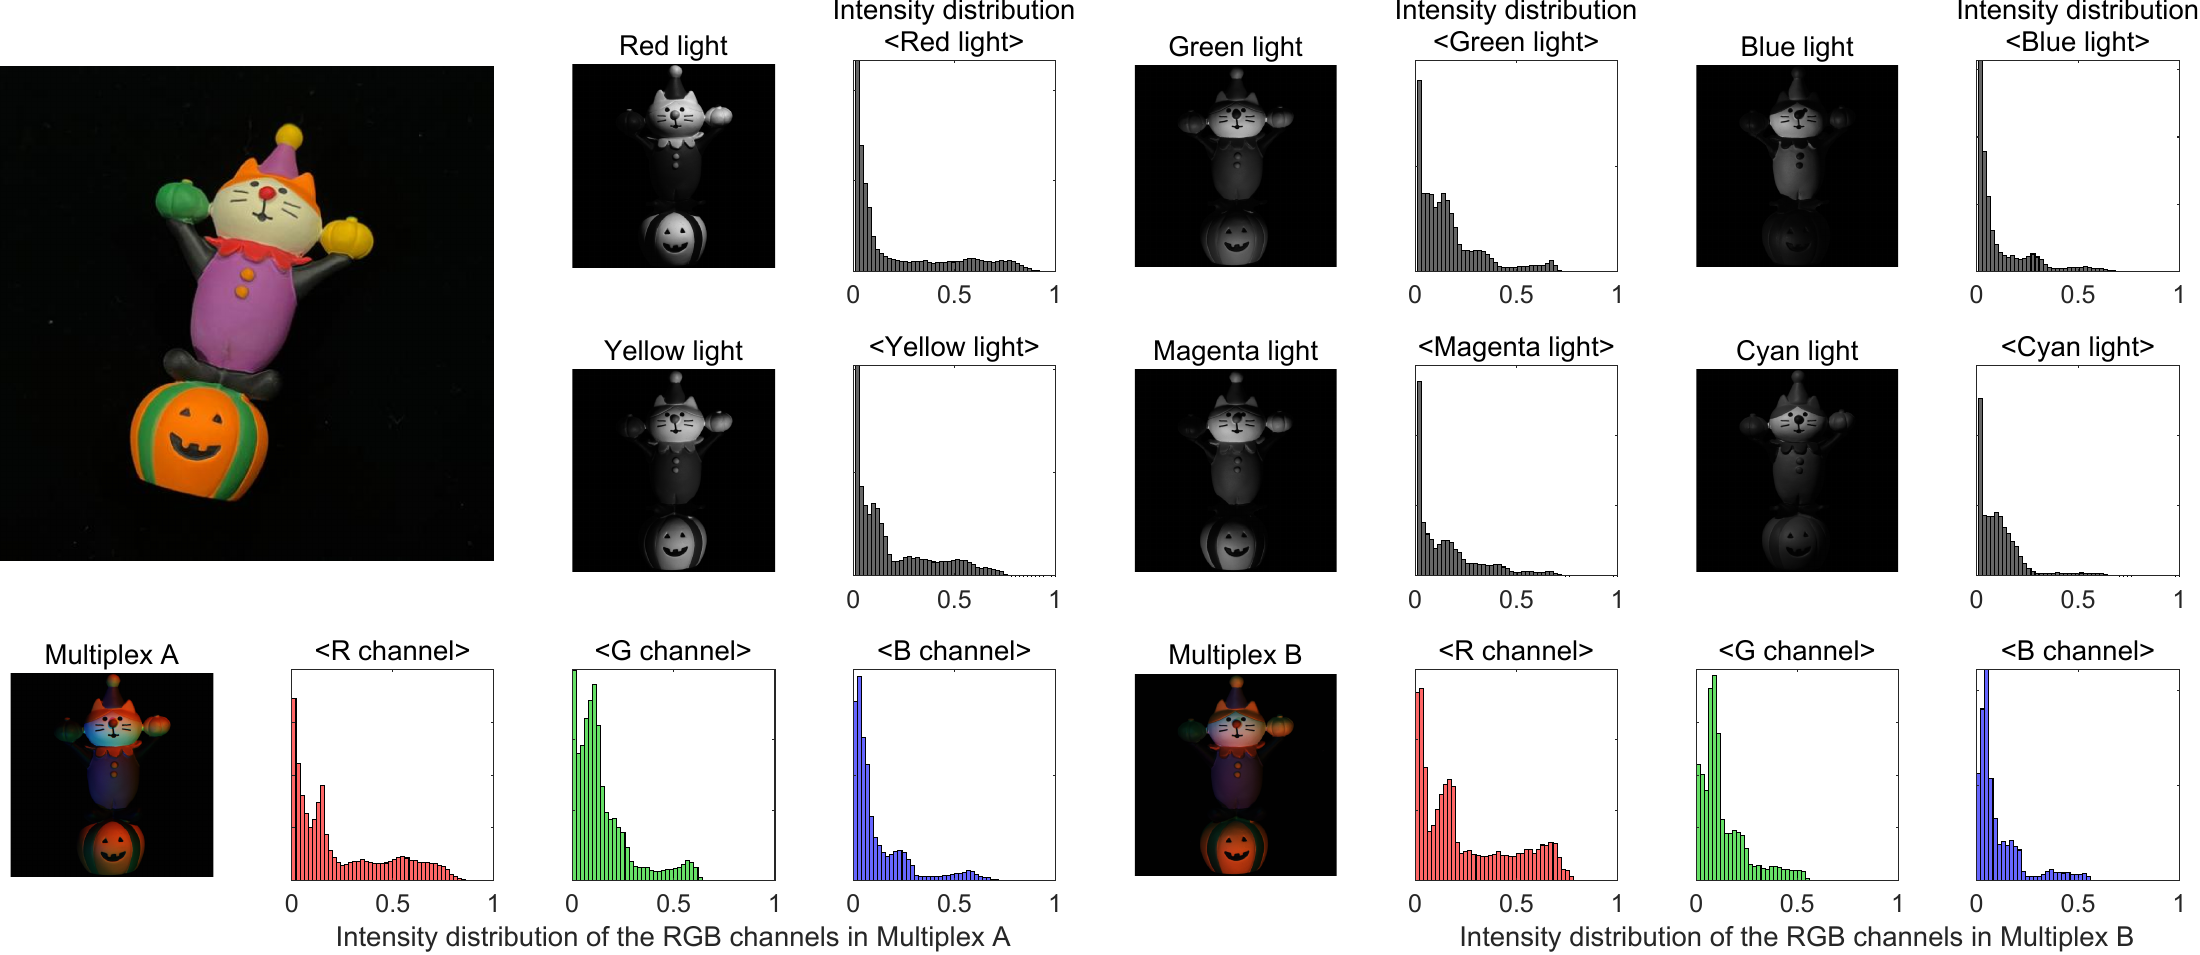}
	\end{center}
	\vspace{-15pt}
	\caption{Crown.
 \protect\linebreak Reflective properties : mostly diffuse.}
	\label{fig:objects_histogram_crown}
	\vspace{-5pt}
\end{figure}

\begin{figure}[h]
	\begin{center}
		\includegraphics[width=120mm]{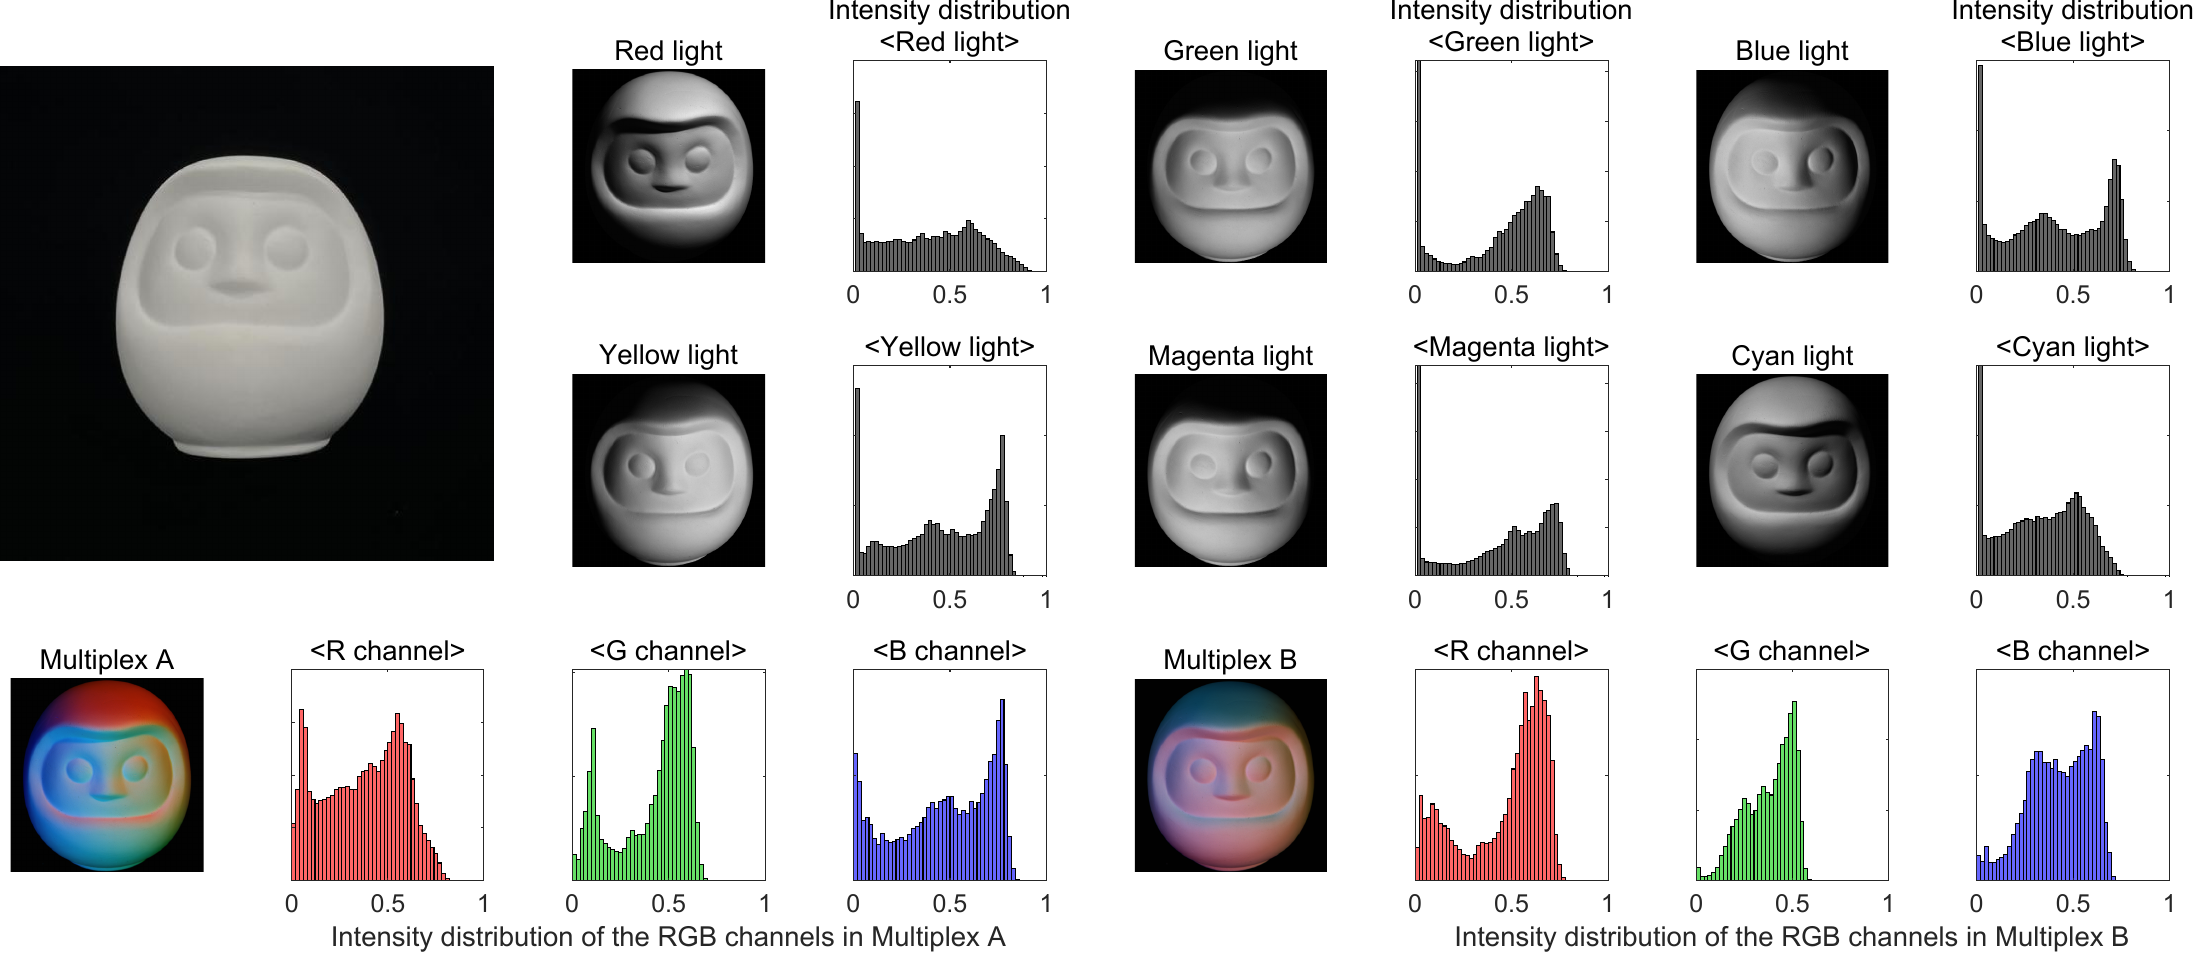}
	\end{center}
	\vspace{-15pt}
	\caption{Daruma.
 \protect\linebreak Reflective properties : mostly diffuse.}
	\label{fig:objects_histogram_daruma}
	\vspace{-5pt}
\end{figure}

% \begin{figure}[h]
% 	\begin{center}
% 		\includegraphics[width=120mm]{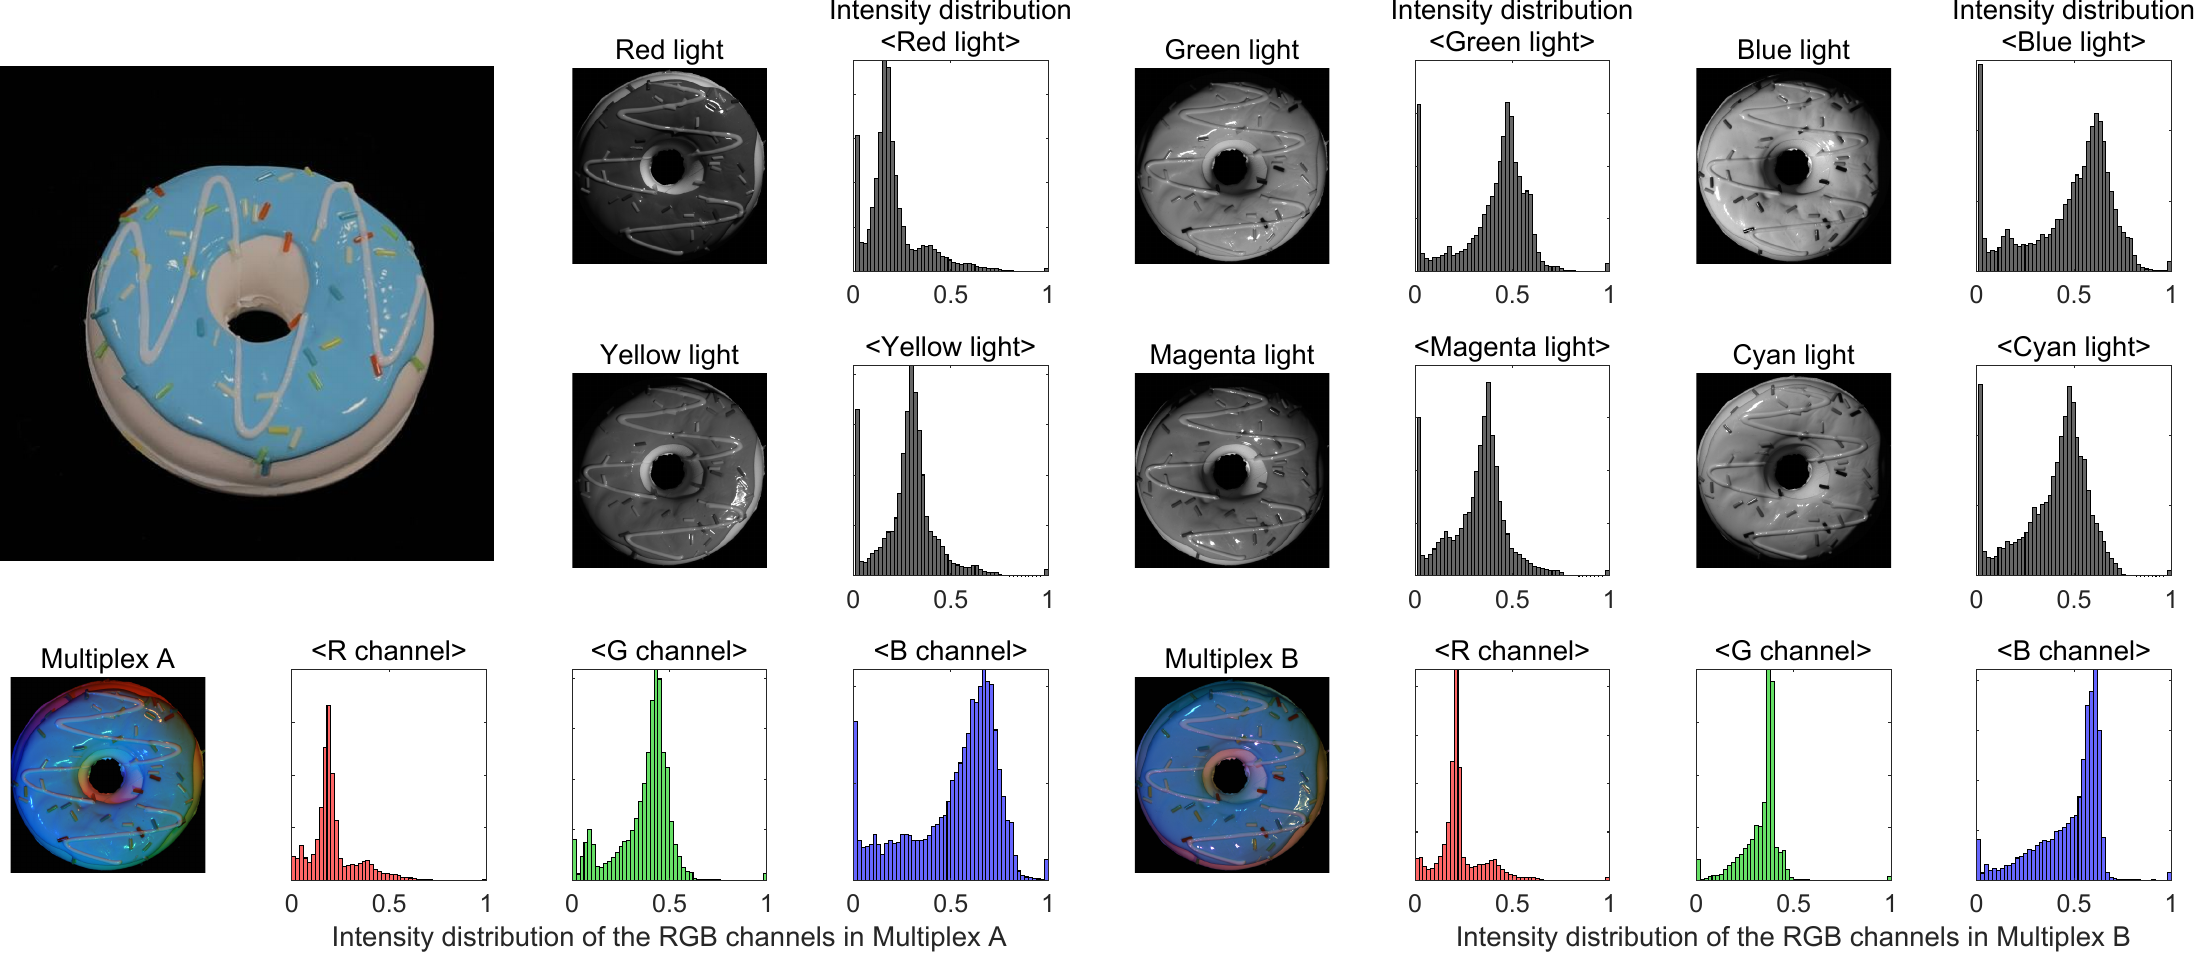}
% 	\end{center}
% 	\vspace{-15pt}
% 	\caption{Donut.
%  \protect\linebreak Reflective properties : diffuse + sparse specular spikes.}
% 	\label{fig:objects_histogram_donut}
% 	\vspace{-5pt}
% \end{figure}

\begin{figure}[h]
	\begin{center}
		\includegraphics[width=120mm]{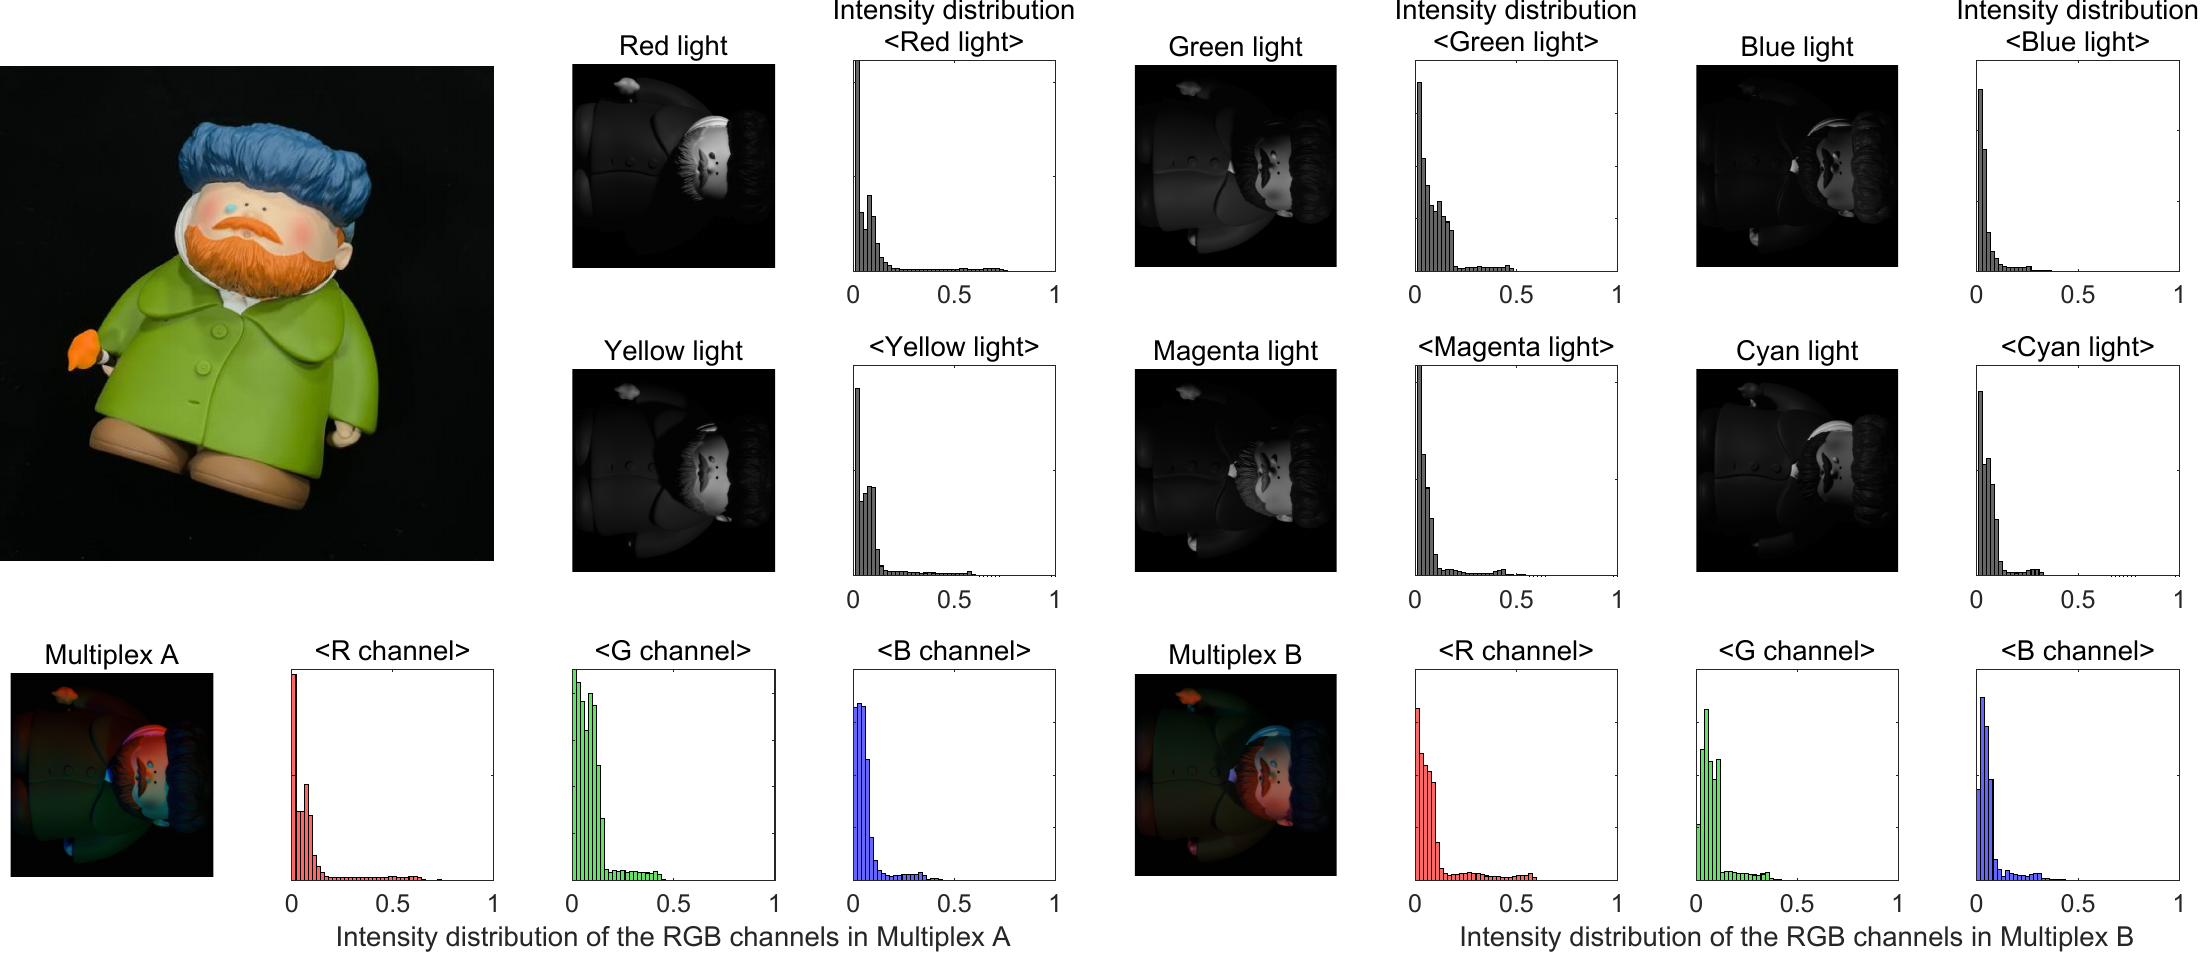}
	\end{center}
	\vspace{-15pt}
	\caption{Gogh.
 \protect\linebreak Reflective properties : mostly diffuse.}
	\label{fig:objects_histogram_gogh}
	\vspace{-5pt}
\end{figure}

\begin{figure}[h]
	\begin{center}
		\includegraphics[width=120mm]{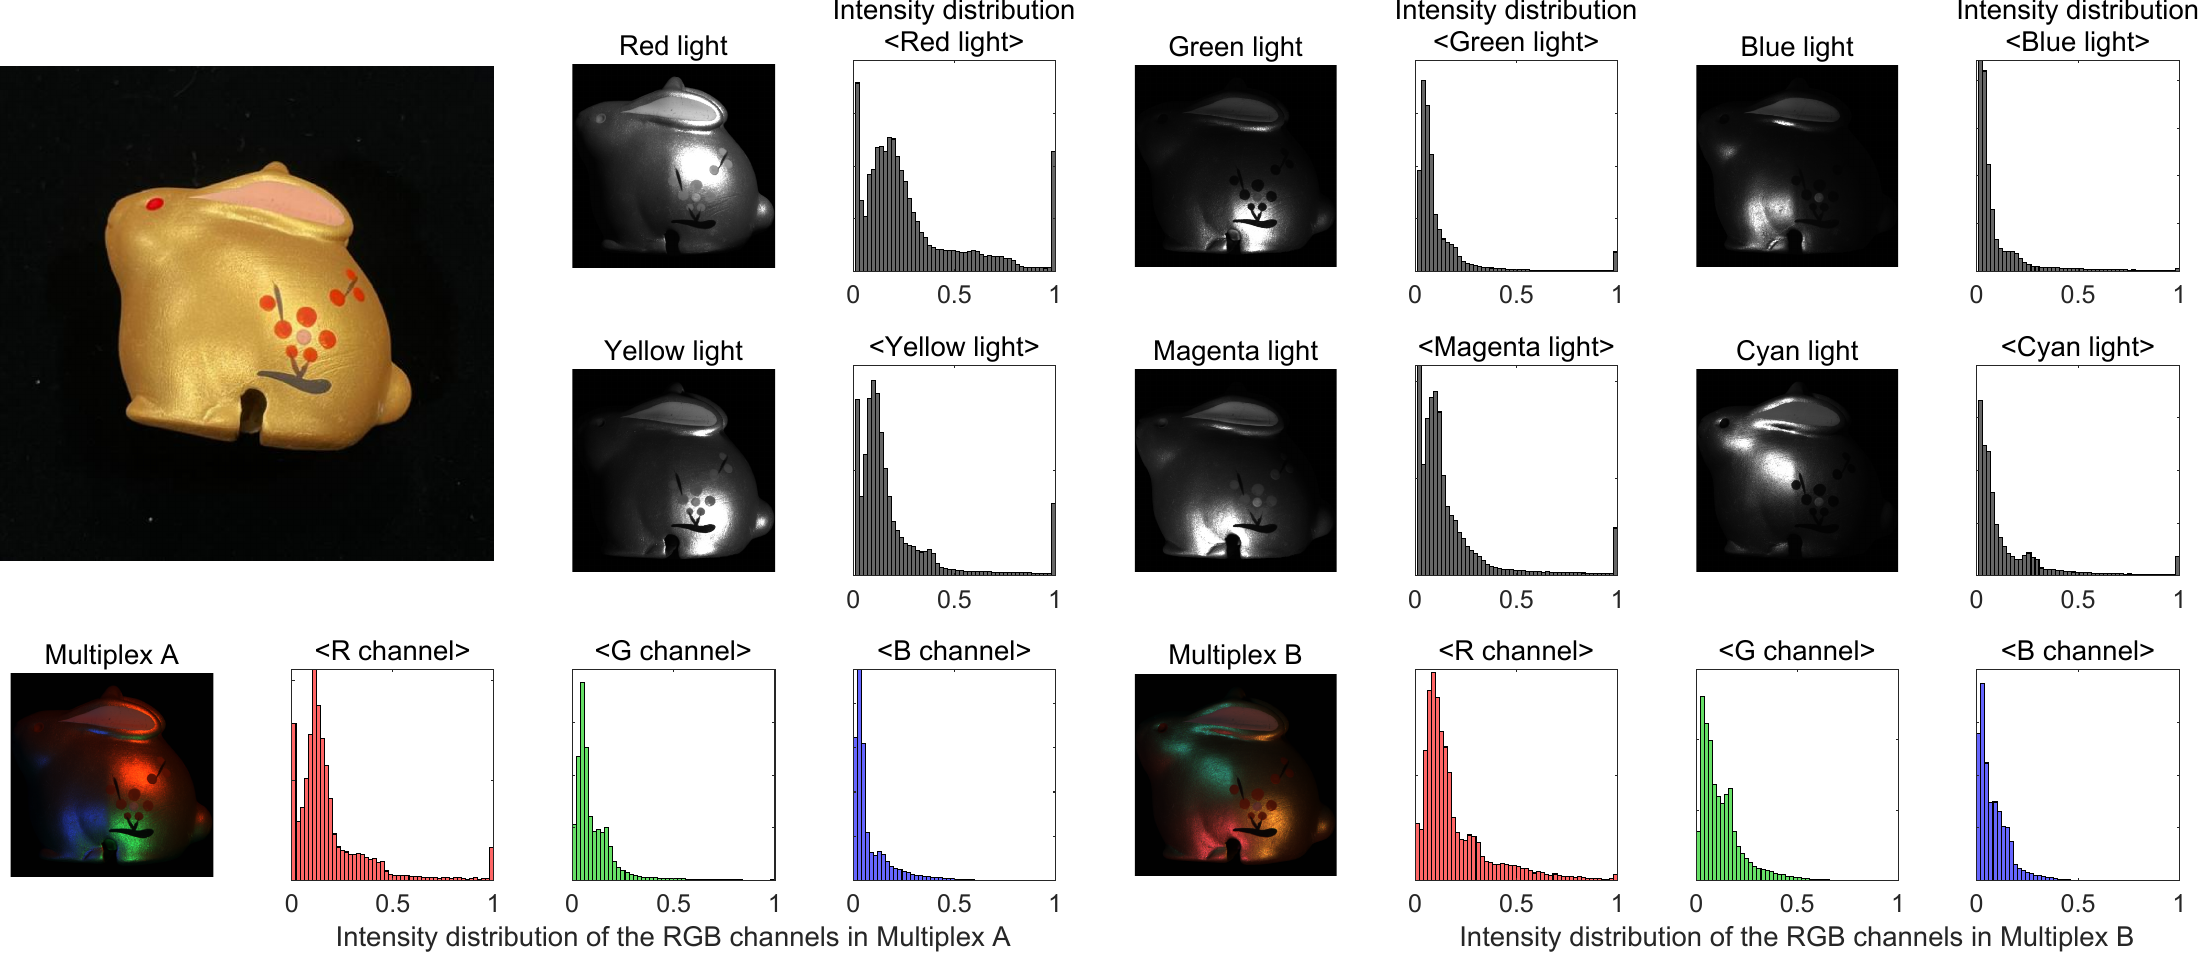}
	\end{center}
	\vspace{-15pt}
	\caption{Golden\_bunny.
 \protect\linebreak Reflective properties : broad and soft specular lobes with metallic paint.}
	\label{fig:objects_histogram_Gbunny}
	\vspace{-5pt}
\end{figure}

\begin{figure}[h]
	\begin{center}
		\includegraphics[width=120mm]{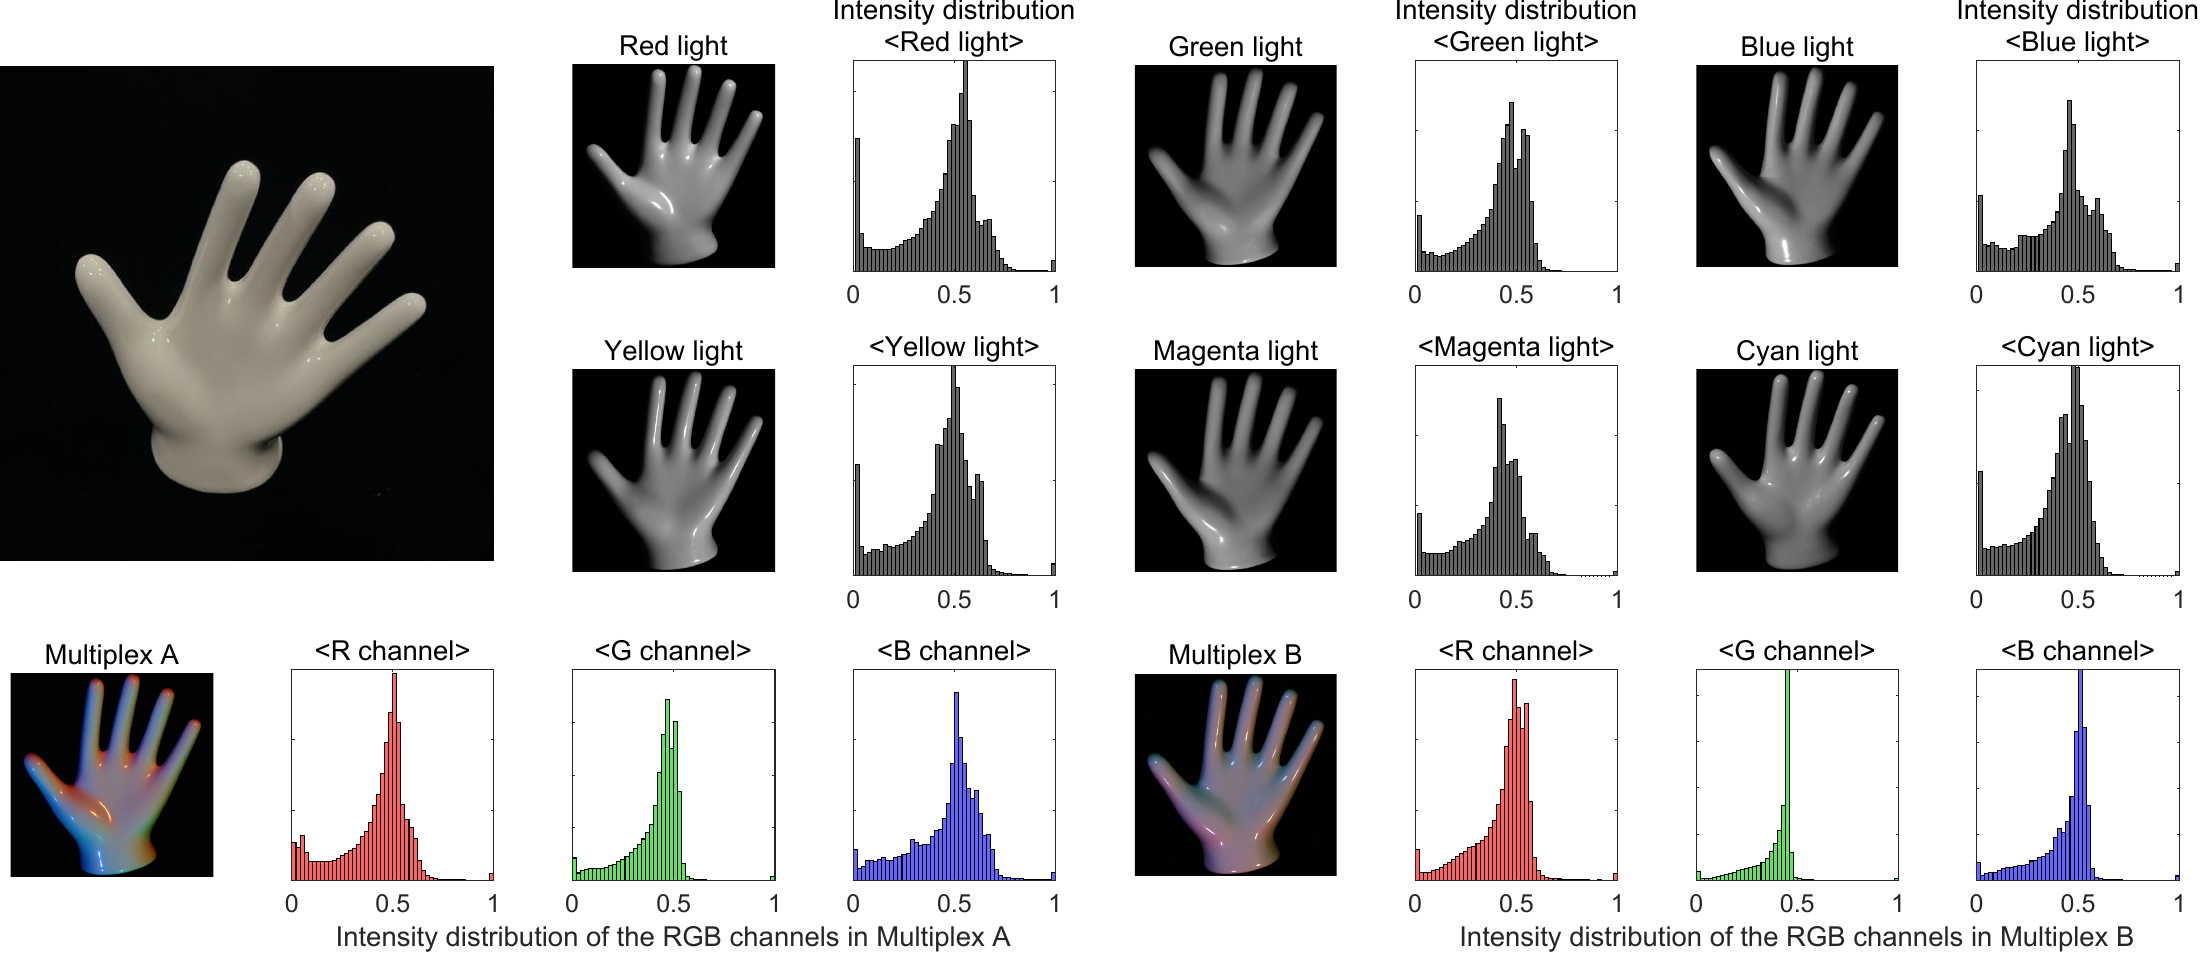}
	\end{center}
	\vspace{-15pt}
	\caption{Hand.
 \protect\linebreak Reflective properties : strong and sparse specular spikes.}
	\label{fig:objects_histogram_hand}
	\vspace{-5pt}
\end{figure}

\begin{figure}[h]
	\begin{center}
		\includegraphics[width=120mm]{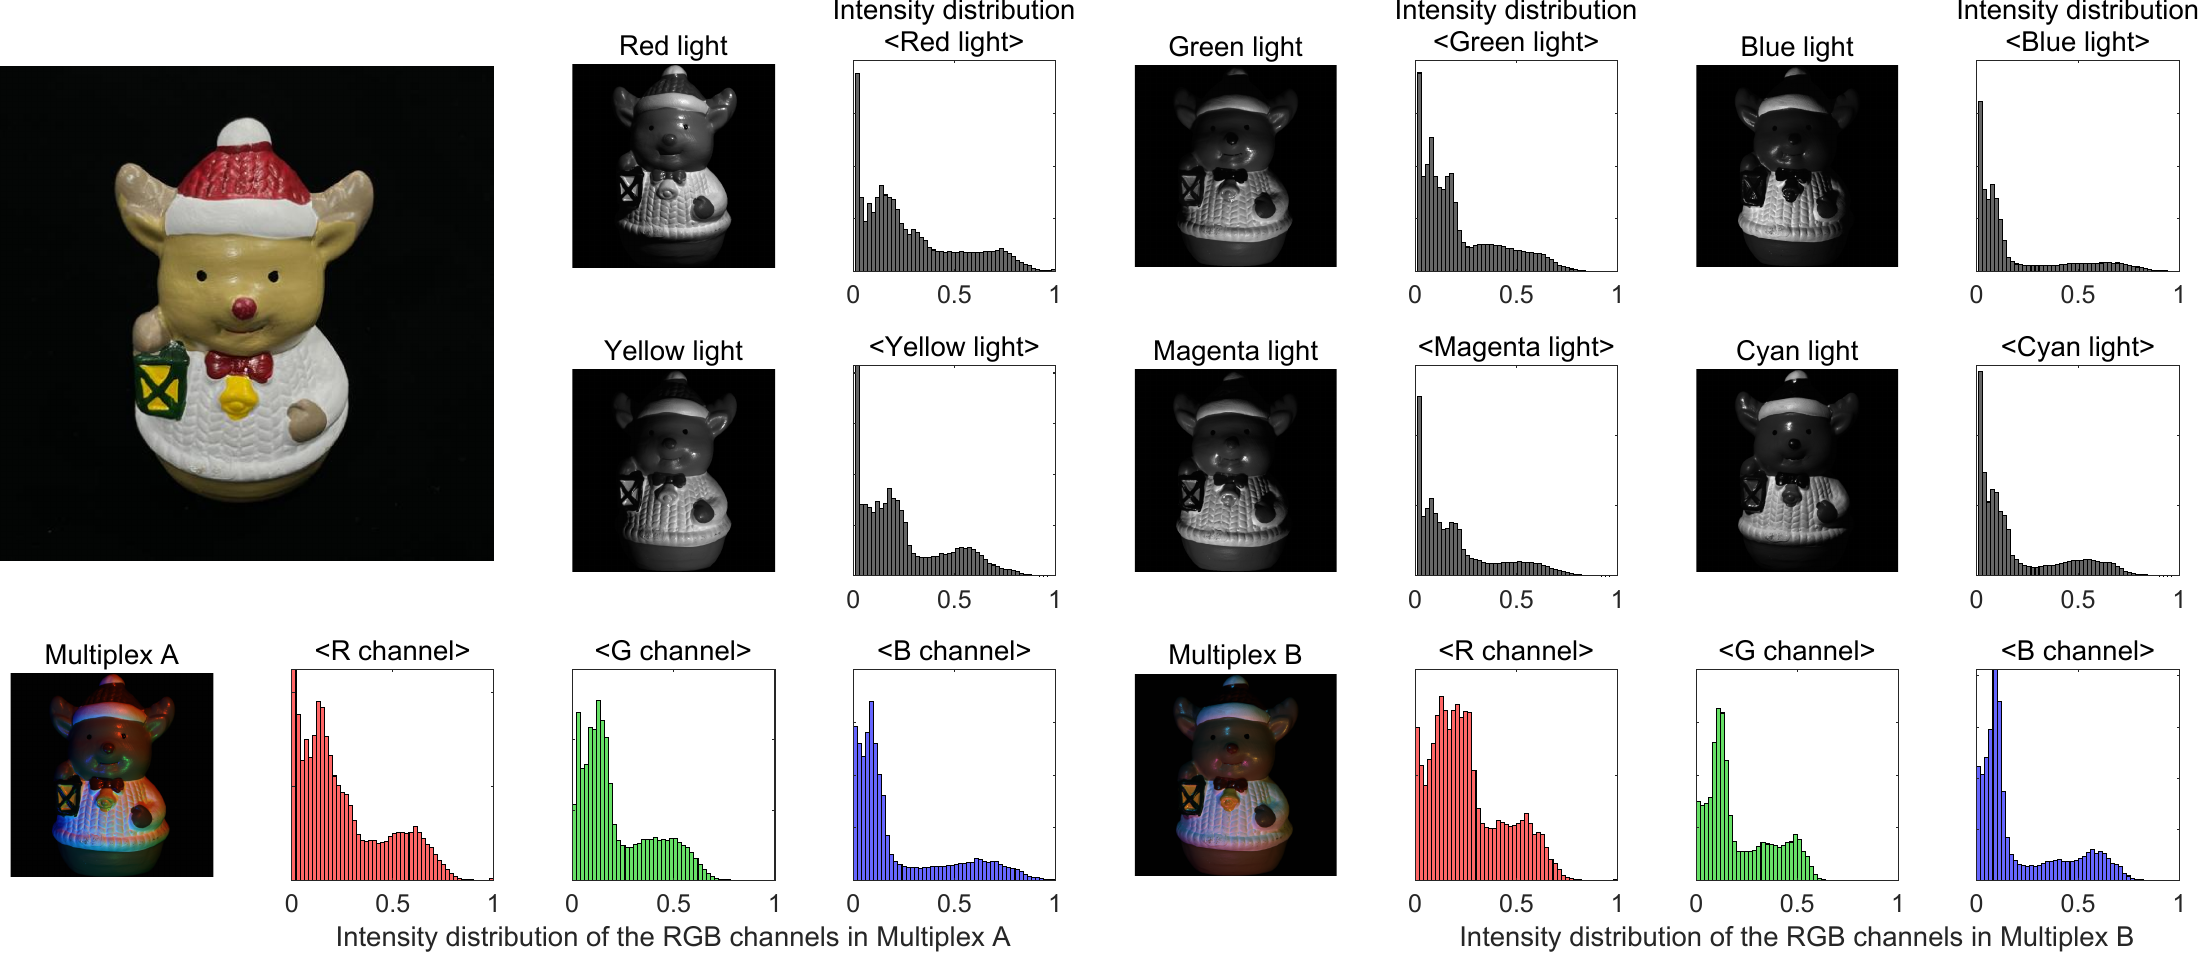}
	\end{center}
	\vspace{-15pt}
	\caption{Reindeer.
 \protect\linebreak Reflective properties : broad and soft specular lobes.}
	\label{fig:objects_histogram_reindeer}
	\vspace{-5pt}
\end{figure}

\begin{figure}[h]
	\begin{center}
		\includegraphics[width=120mm]{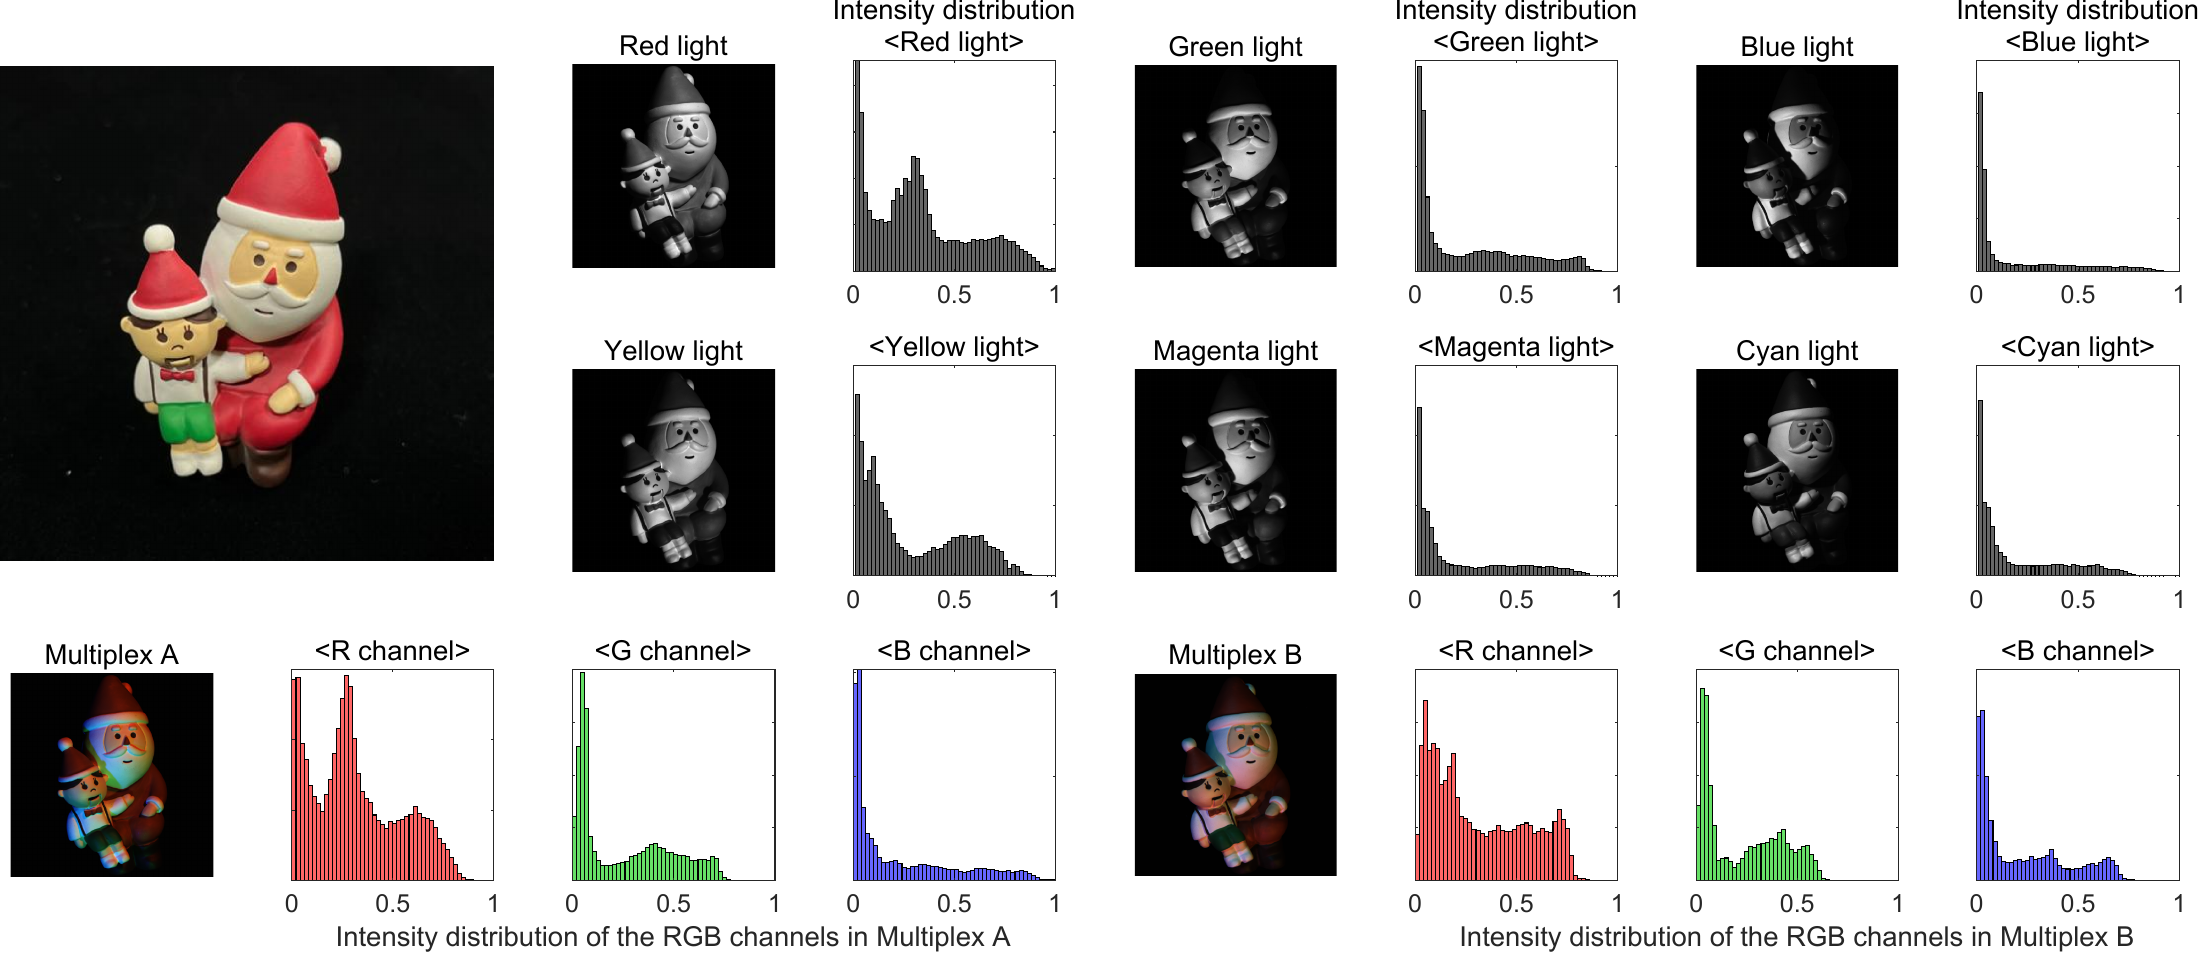}
	\end{center}
	\vspace{-15pt}
	\caption{Santa.
 \protect\linebreak Reflective properties : mostly diffuse.}
	\label{fig:objects_histogram_santa}
	\vspace{-5pt}
\end{figure}

\begin{figure}[h]
	\begin{center}
		\includegraphics[width=120mm]{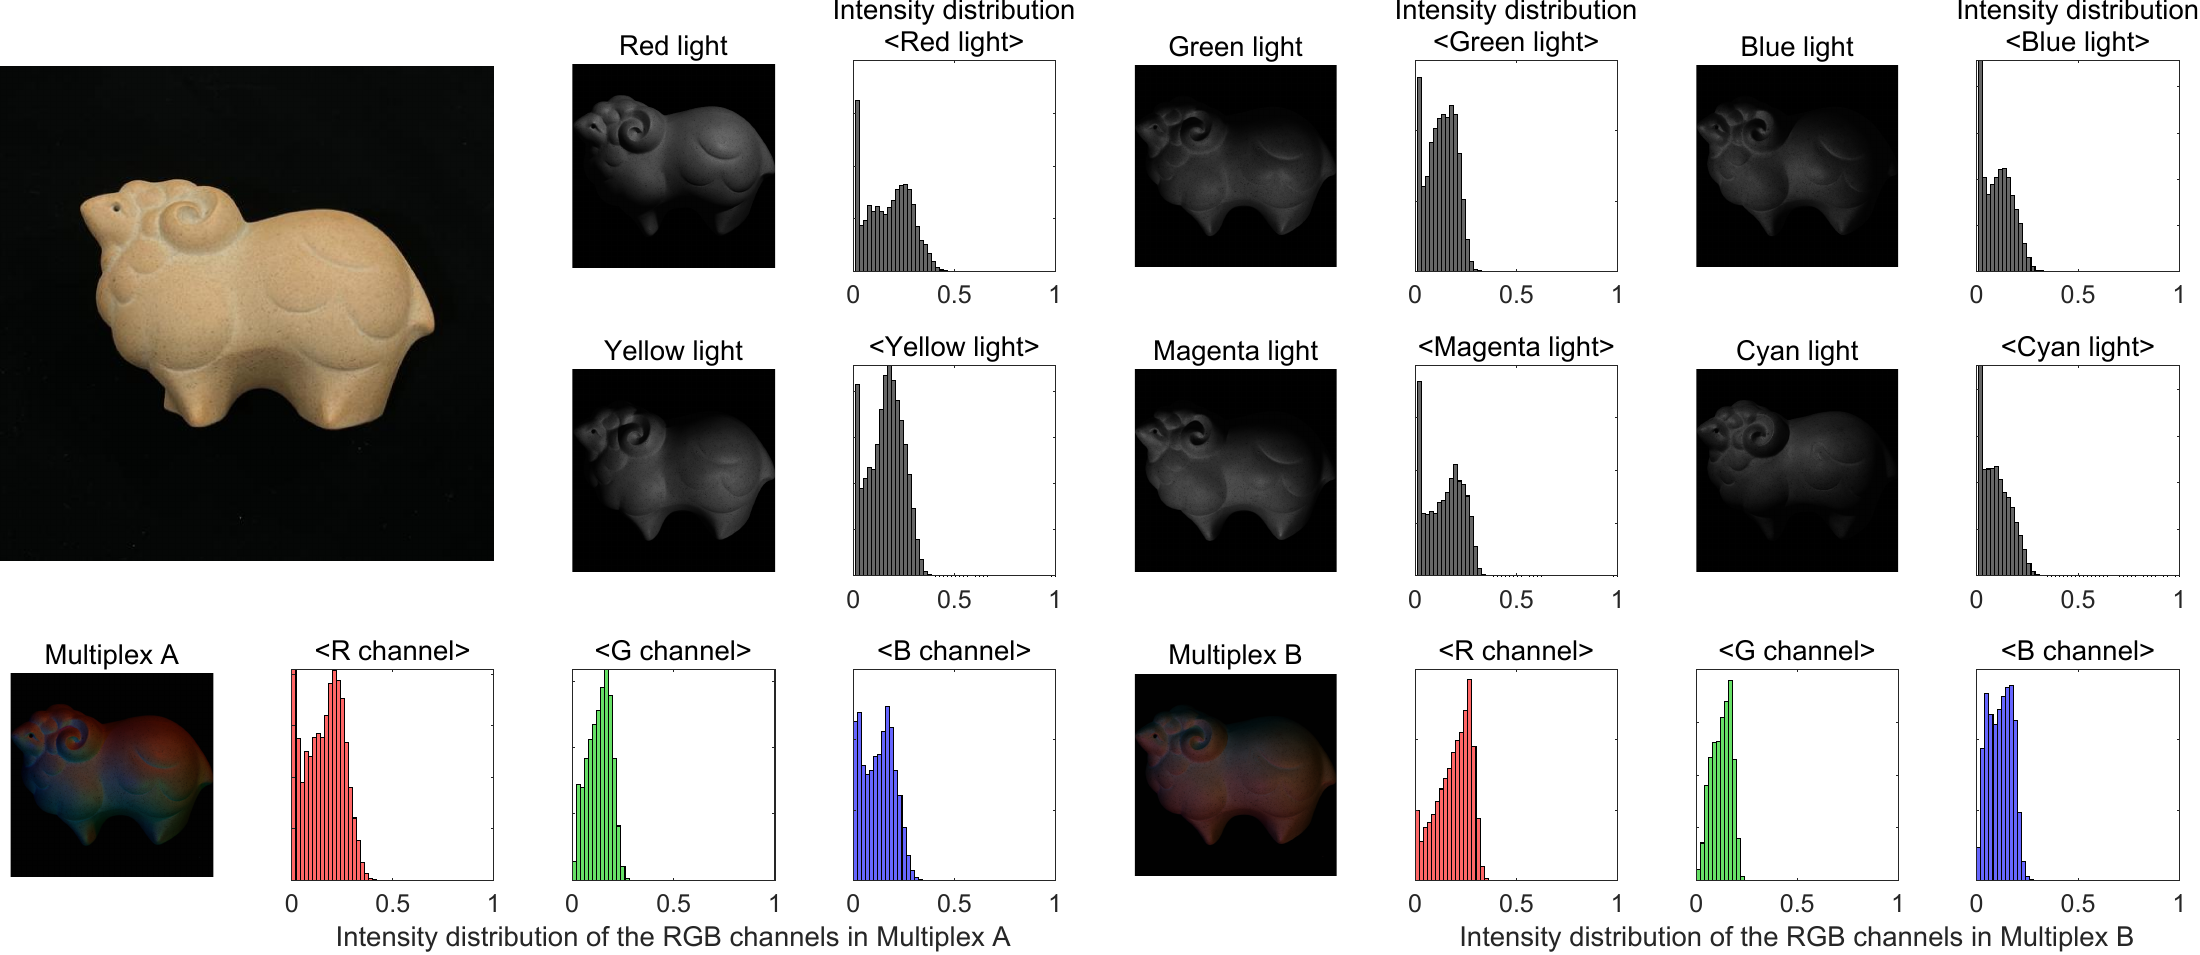}
	\end{center}
	\vspace{-15pt}
	\caption{Sheep.
 \protect\linebreak Reflective properties : mostly diffuse.}
	\label{fig:objects_histogram_sheep}
	\vspace{-5pt}
\end{figure}

\begin{figure}[h]
	\begin{center}
		\includegraphics[width=120mm]{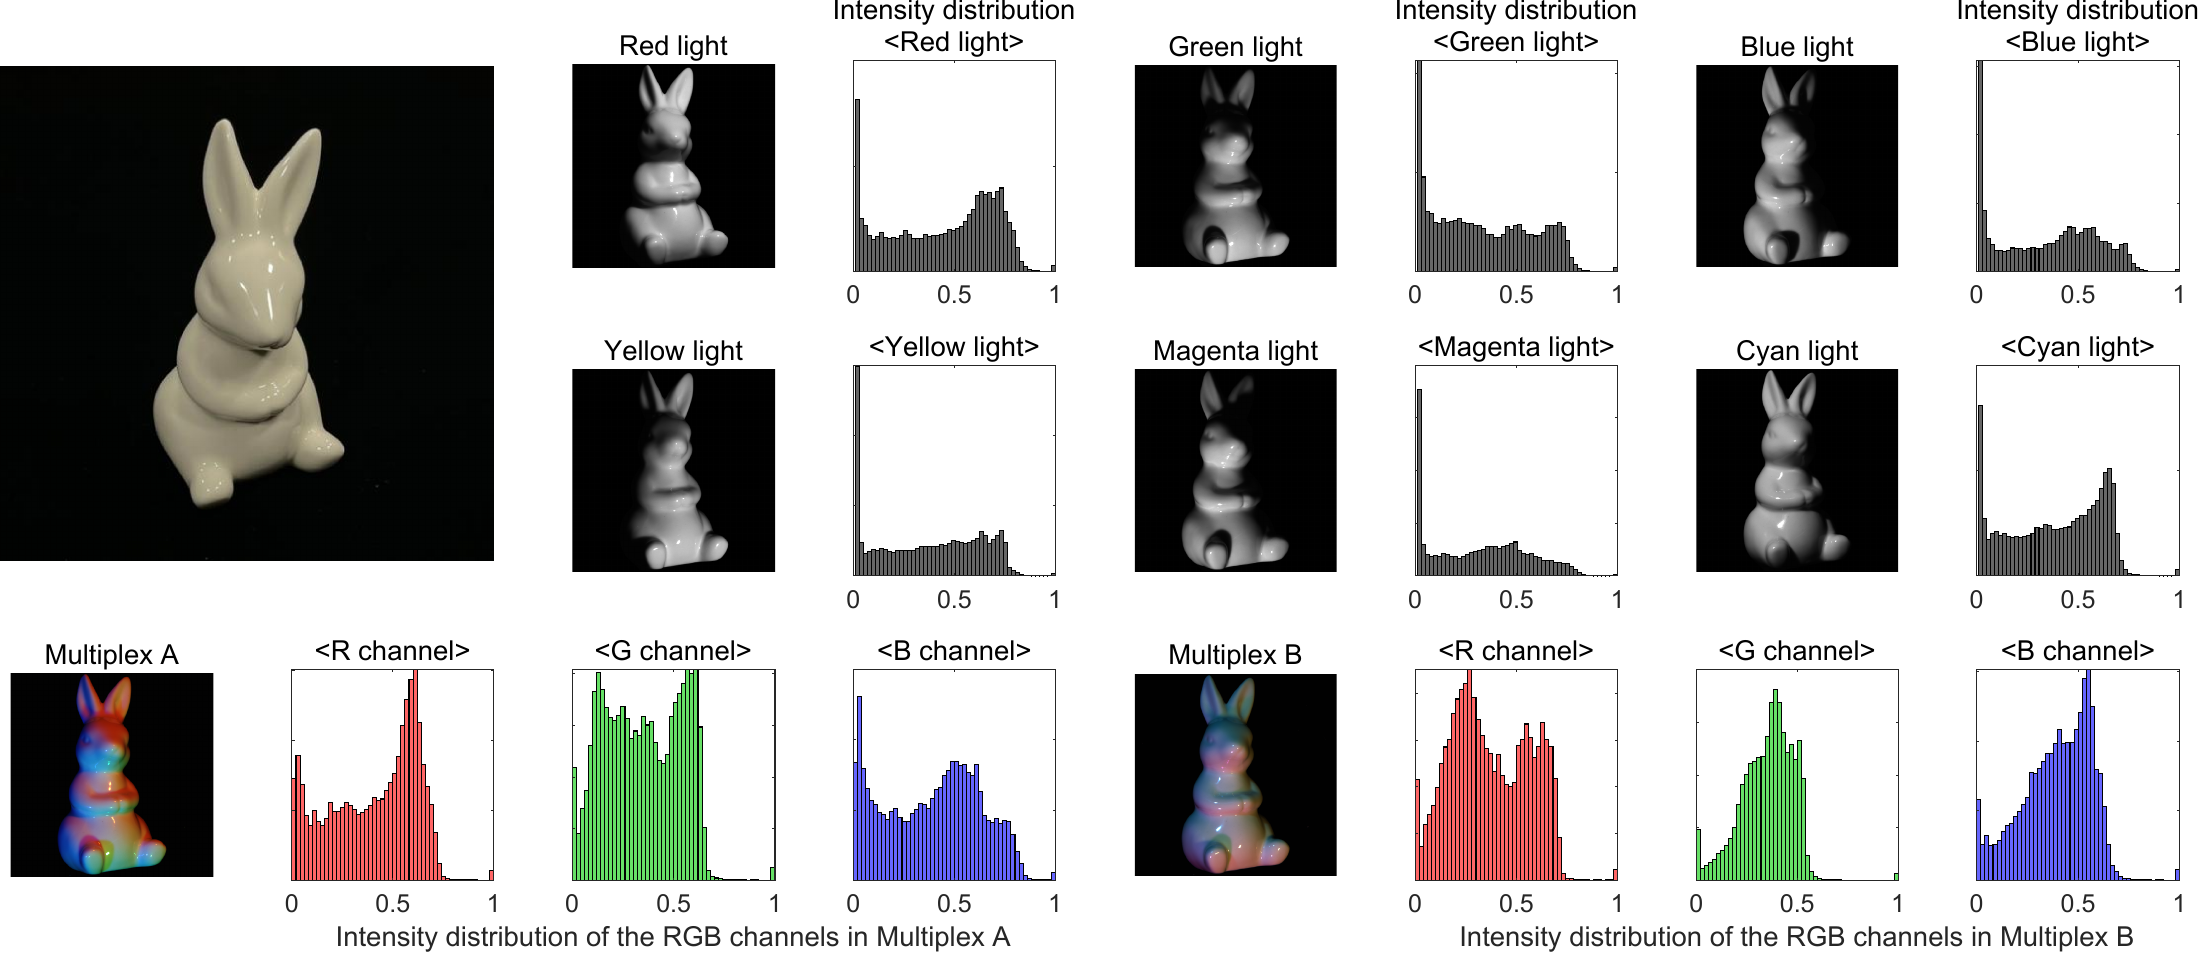}
	\end{center}
	\vspace{-15pt}
	\caption{White\_bunny.
 \protect\linebreak Reflective properties : strong and sparse specular spikes.}
	\label{fig:objects_histogram_White_bunny}
	\vspace{-5pt}
\end{figure}

\begin{figure}[h]
	\begin{center}
		\includegraphics[width=120mm]{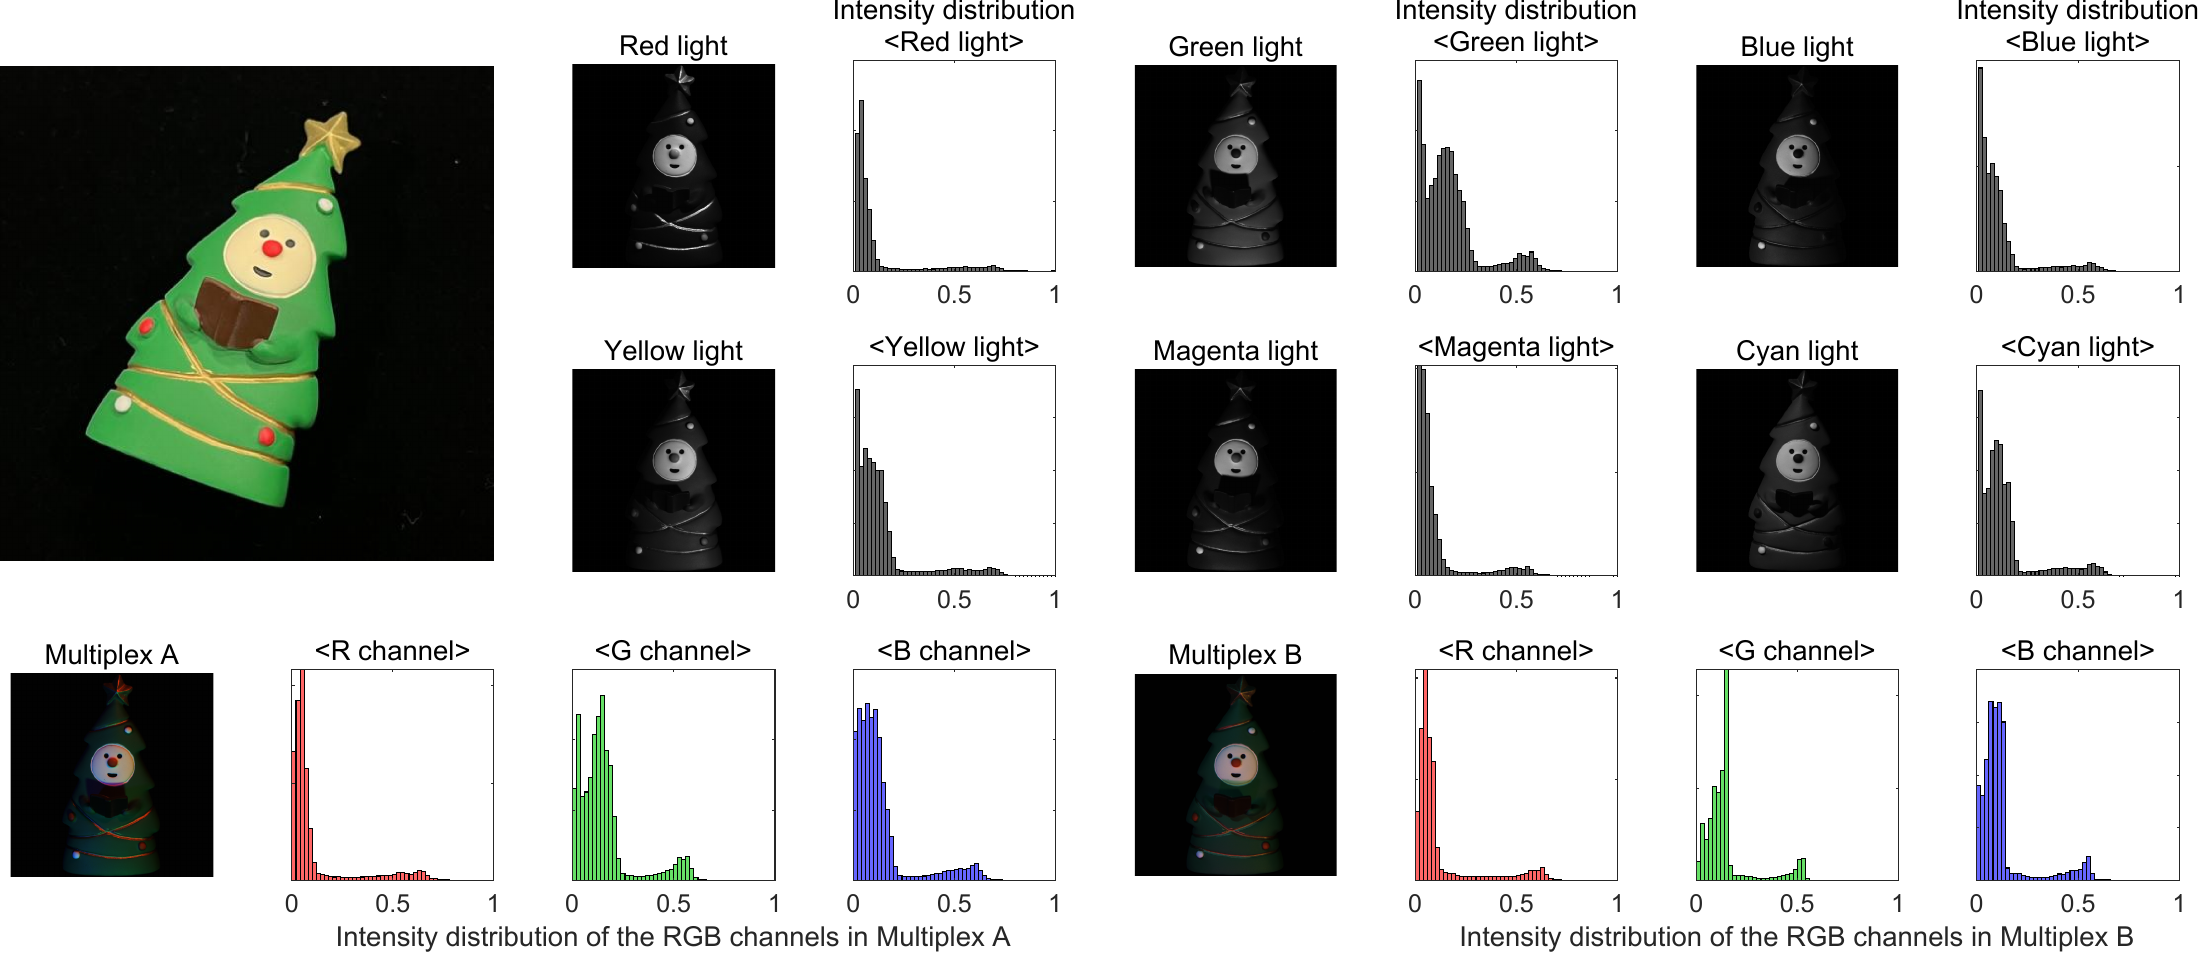}
	\end{center}
	\vspace{-15pt}
	\caption{Tree.
 \protect\linebreak Reflective properties : mostly diffuse.}
	\label{fig:objects_histogram_tree}
	\vspace{-5pt}
\end{figure}
